# Supplementary material for: Multi-Objective Alignment of Language Models for Personalized Psychotherapy
Source: arXiv:2602.16053 source file (2026-02-17)
Supplement: Supplementary file 1 [file supplementary.tex]

\subsection{Technical Foundation: From RLHF to Multi-Objective DPO}

Current approaches to AI alignment in healthcare predominantly employ single-objective optimization, typically focusing on either helpfulness or safety. However, the complexity of therapeutic relationships involves multiple, often competing objectives: building trust while maintaining boundaries, providing empathy while ensuring accuracy, offering validation while challenging maladaptive thoughts, and maintaining engagement while respecting autonomy. Traditional alignment methods fail to capture these nuanced trade-offs that characterize effective psychotherapy~\cite{shen2024bidirectional}.

The technical foundation for addressing these challenges has evolved significantly with the development of Direct Preference Optimization (DPO) as an alternative to Reinforcement Learning from Human Feedback (RLHF). While standard DPO addresses single-objective alignment, recent multi-objective extensions offer promising directions for therapeutic communication's complex requirements. Traditional RLHF approaches involve a complex multi-stage process: first training a reward model to predict human preferences from comparison data, then using reinforcement learning algorithms like Proximal Policy Optimization (PPO) to fine-tune the language model to maximize this learned reward while maintaining similarity to the original model through KL-divergence constraints~\cite{ouyang2022training,schulman2017proximal}. This process requires careful hyperparameter tuning, can be unstable during training, and necessitates repeated sampling from the model during optimization.

DPO fundamentally reimagines this process by recognizing that the optimal policy can be derived analytically from the reward model, eliminating the need for reinforcement learning entirely~\cite{rafailov2023direct}. Instead of the multi-stage RLHF pipeline, DPO directly optimizes the language model using a simple classification loss on preference pairs, making it an "offline" method that requires only the original preference dataset without additional sampling or reward model training. This approach offers substantial practical advantages: improved training stability, reduced computational overhead, and elimination of the complex hyperparameter tuning associated with RL algorithms.

Multi-Objective Direct Preference Optimization (MODPO) extends these benefits to enable simultaneous optimization across multiple therapeutic objectives with significantly reduced computational requirements compared to traditional multi-objective approaches~\cite{zhou2024modpo}. This technical advance is particularly relevant for psychotherapy applications, where systems must balance competing therapeutic goals while adapting to individual patient preferences and therapeutic contexts.

\subsection{Evaluation Methodology and Synthetic Personas}

Validation of personalized AI systems requires methodological innovations that can assess performance across diverse patient populations while addressing the ethical and practical constraints of mental health research. Synthetic persona-based evaluation has emerged as a promising approach, with recent research demonstrating that LLM-generated personas show comparable validity to human-users~\cite{argyle2023out}. This methodology enables systematic evaluation across diverse demographic groups, cultural backgrounds, and therapeutic preferences while maintaining research efficiency and ethical standards.

\subsection{Additional Related Work}

The development of effective therapeutic AI systems requires addressing fundamental challenges in multi-objective optimization, domain-specific alignment, and evaluation methodology. This work builds upon recent advances in these interconnected areas while identifying critical gaps in current approaches.

\subsection{Multi-Objective Alignment for Language Models}

Traditional RLHF approaches optimize language models for single objectives or treat multiple objectives as averaged preferences, failing to capture the diverse and often conflicting nature of human needs. Zhou et al. \cite{zhou2024modpo} addressed this limitation by introducing Multi-Objective Direct Preference Optimization (MODPO), which extends DPO to handle multiple alignment objectives simultaneously. MODPO trains language models as implicit collective reward models that combine objectives with specific weights, theoretically yielding the same optimal solutions as multi-objective RLHF while being three times more computationally efficient. However, their work focuses on general alignment objectives (helpfulness vs. harmlessness) rather than specialized domains.

Building on multi-objective concepts, Jang et al. \cite{jang2023personalized} developed Personalized Soups, demonstrating that models trained on different objectives can be effectively combined through parameter merging during inference. Their approach reduces computational complexity from exponential to linear in the number of preferences and models alignment as a Multi-Objective Reinforcement Learning problem where preferences are decomposed into multiple dimensions. While promising for general preferences, neither MODPO nor Personalized Soups has been applied to therapeutic contexts where objectives like empathy, trust, and autonomy require careful balancing.

The broader field of Multi-Objective Reinforcement Learning (MORL) has demonstrated effectiveness in healthcare contexts, including resource allocation and planning applications \cite{mosavi2022multi,felten2024multi}. These studies show that MORL can effectively balance competing healthcare objectives, though they focus on operational rather than communicative aspects of healthcare delivery.

\subsection{Therapeutic AI and Mental Health Applications}
\begin{comment}
Recent clinical validation has demonstrated the potential of AI-powered therapeutic interventions. Heinz et al. \cite{heinz2025randomized} conducted the first randomized controlled trial of a generative AI therapy chatbot, showing substantial symptom reductions: 51\% for depression, 31\% for anxiety, and 19\% for eating disorders. 

Participants rated therapeutic alliance with the AI as comparable to human therapists, establishing clinical feasibility. However, their approach employed a single therapeutic framework based on third-wave CBT, integrating empirically grounded contextual and functional approaches without addressing the multi-objective optimization challenges inherent in therapeutic communication.
\end{comment}
Most current therapeutic AI research focuses on single objectives, particularly empathy enhancement. Chen et al. \cite{chen2023soulchat} developed SoulChat using over 2 million empathetic conversation samples, demonstrating significant improvements in empathy-related responses. However, they explicitly acknowledge conflicts between therapeutic objectives, noting that "there may be a certain conflict between Empathy and Helpfulness" where ChatGPT tends to generate helpful but less empathetic responses. This tension highlights the need for systematic multi-objective approaches rather than single-objective optimization.

Lee et al. \cite{lee2024chain} proposed Chain of Empathy prompting, incorporating insights from multiple psychotherapy frameworks (CBT, DBT, Person Centered Therapy, Reality Therapy) to enhance empathetic responses. While their work demonstrates the value of psychotherapy-informed approaches, it relies on prompting strategies rather than training-time optimization, limiting its ability to systematically balance competing therapeutic objectives.

Research on LLM therapeutic behavior has revealed concerning patterns in current alignment approaches. Studies show that RLHF-trained models exhibit excessive problem-solving behaviors similar to low-quality human therapy, as RLHF's focus on helpfulness leads models to over-emphasize solution provision even in therapeutic contexts \cite{chiu2024computational}. This finding underscores the inadequacy of general-purpose alignment for therapeutic applications.

\subsection{Evaluation Challenges and Synthetic Methodologies}

Evaluating therapeutic AI presents unique challenges due to ethical constraints on involving vulnerable populations and the multidimensional nature of therapeutic effectiveness. Recent advances in synthetic evaluation provide promising solutions. Argyle et al. \cite{argyle2023out} demonstrated that LLM-generated personas achieve comparable validity to human-created ones in user studies, establishing the foundation for persona-based evaluation methodologies. Building on this, Louie et al. \cite{louie2024roleplay} developed Roleplay-doh, enabling domain experts to create behaviorally authentic patient representations through principle-based persona generation.

These methodological advances have been extended to therapeutic contexts. Wang et al. \cite{wang2024patient} developed Patient-Ψ for training mental health professionals using LLM-simulated patients with cognitive modeling, demonstrating realistic patient behaviors. However, existing synthetic evaluation approaches focus on training applications rather than systematic therapeutic AI alignment assessment. The validation of synthetic evaluation against human judgment specifically for therapeutic AI remains unexplored.

\subsection{Domain-Specific vs. General Communication Principles}

The question of whether specialized domains require domain-specific optimization or can rely on adapted general principles remains unresolved. While Grice's conversational maxims \cite{grice1975logic}—quantity, quality, relation, and manner—establish fundamental communication effectiveness principles, therapeutic communication often requires departures from these norms. Therapeutic contexts may require providing emotional support over factual accuracy, addressing feelings rather than logical relevance, and using communication styles that prioritize patient comfort over efficiency.

Despite extensive research in both therapeutic communication theory and general communication frameworks, no systematic empirical comparison exists between domain-specific therapeutic criteria and adapted general communication principles for AI alignment. This gap represents a critical missing piece in understanding whether therapeutic AI requires specialized optimization approaches.

This work builds upon these advances to develop multi-objective therapeutic AI alignment through systematic integration of MODPO with domain-specific therapeutic criteria and validated synthetic evaluation methodologies.

\subsection{Demographic Distribution of Patient Survey}
\label{appendix:demographic_distr}

The complete persona pool (n=335) demonstrated substantial demographic diversity essential for comprehensive therapeutic AI evaluation (Figure~\ref{fig:demographics}). Age distribution showed concentration in young adult populations (18-24: 37.6\%; 25-34: 23.6\%), with meaningful representation across older age groups (35-44: 19.4\%; 45-54: 10.4\%; 55+: 7.2\%). Gender representation included female (61.5\%), male (34.3\%), and non-binary (2.7\%) participants. Ethnicity distribution achieved balanced representation across major groups: White/Caucasian (30.4\%), Black/African American (29.6\%), Asian (27.8\%), Hispanic/Latino (6.3\%), Middle Eastern/North African (3.0\%), with remaining participants (3.0\%) classified as Others.

We compare between the training set and test set. Ethnicity distribution showed minimal deviation: Asian (Train: 32.0\% vs. Test: 30.0\%), Black/African American (Train: 29.0\% vs. Test: 28.0\%), White/Caucasian (Train: 26.0\% vs. Test: 32.0\%), with other groups maintaining proportional representation. Gender distribution remained consistent (Female—Train: 50.0\% vs. Test: 54.0\%; Male—Train: 46.0\% vs. Test: 38.0\%; Non-binary—Train: 3.0\% vs. Test: 8.0\%). Age distribution similarly preserved proportions across both sets, ensuring that model evaluation would not be confounded by demographic imbalances between training and test populations.
% Figure 1: Demographics composition (combined)
\begin{figure}[htbp]
    \centering
    \begin{subfigure}[b]{0.6\textwidth}
        \centering
        \includegraphics[width=\textwidth]{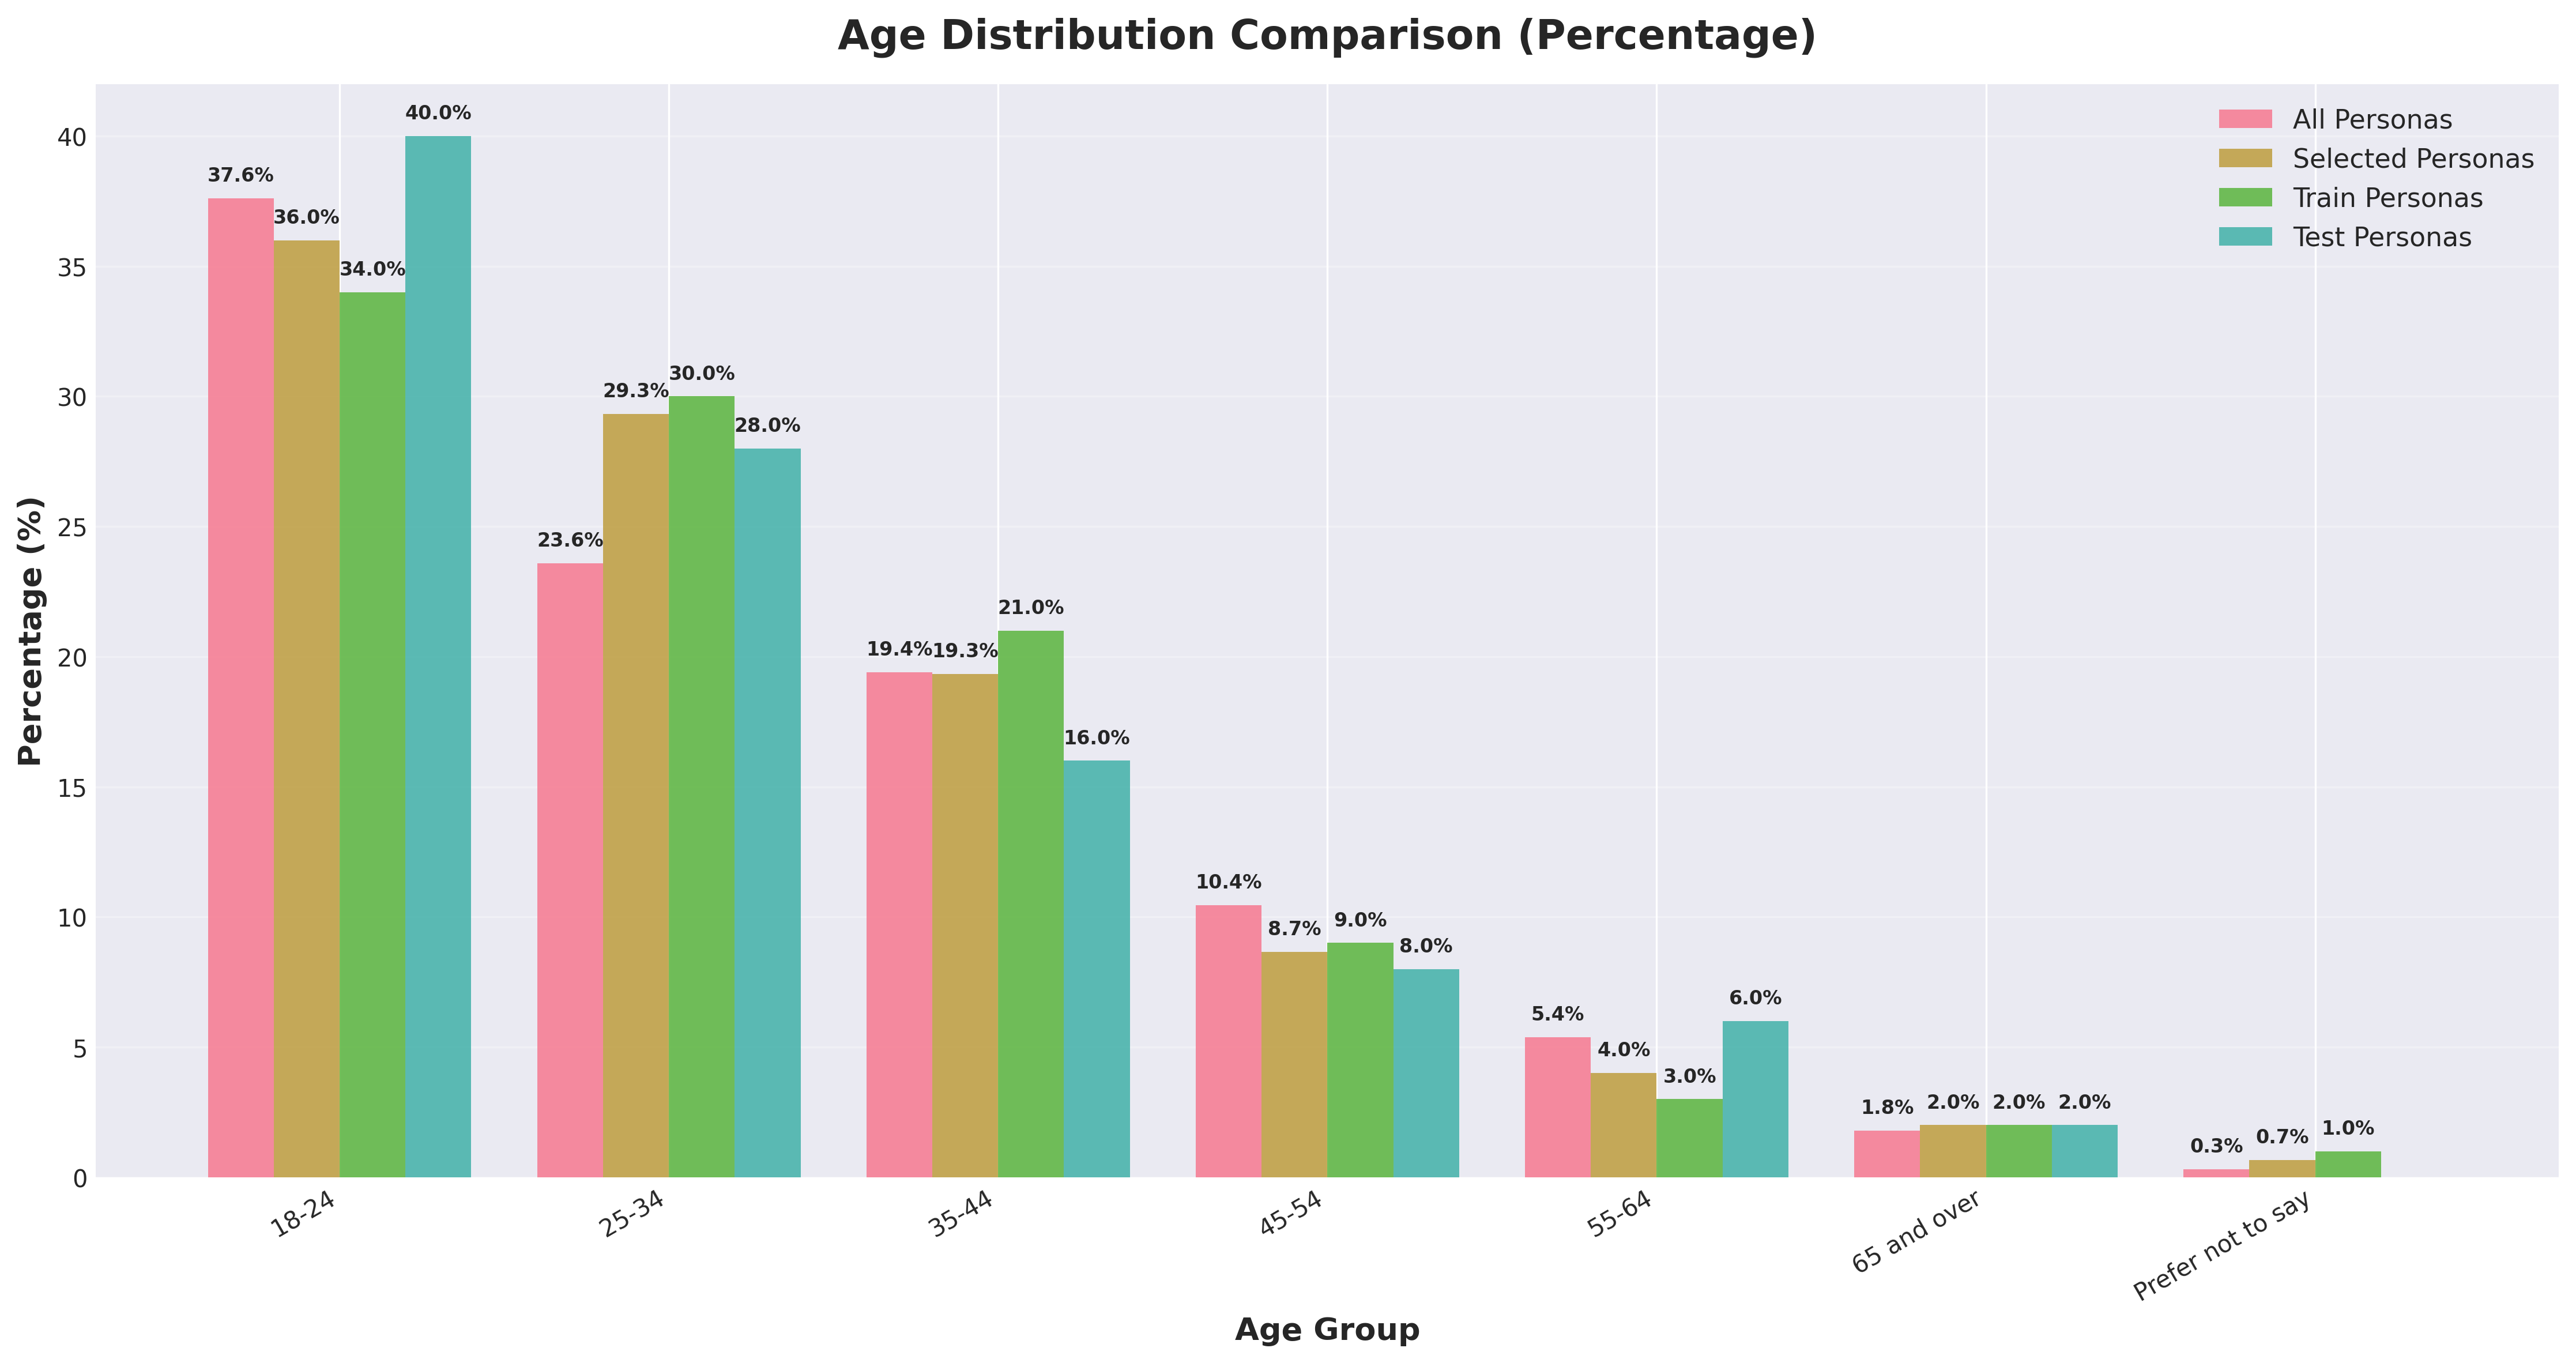}
        \caption{Age distribution}
        \label{fig:demographics_age}
    \end{subfigure}
    
    \begin{subfigure}[b]{0.6\textwidth}
        \centering
        \includegraphics[width=\textwidth]{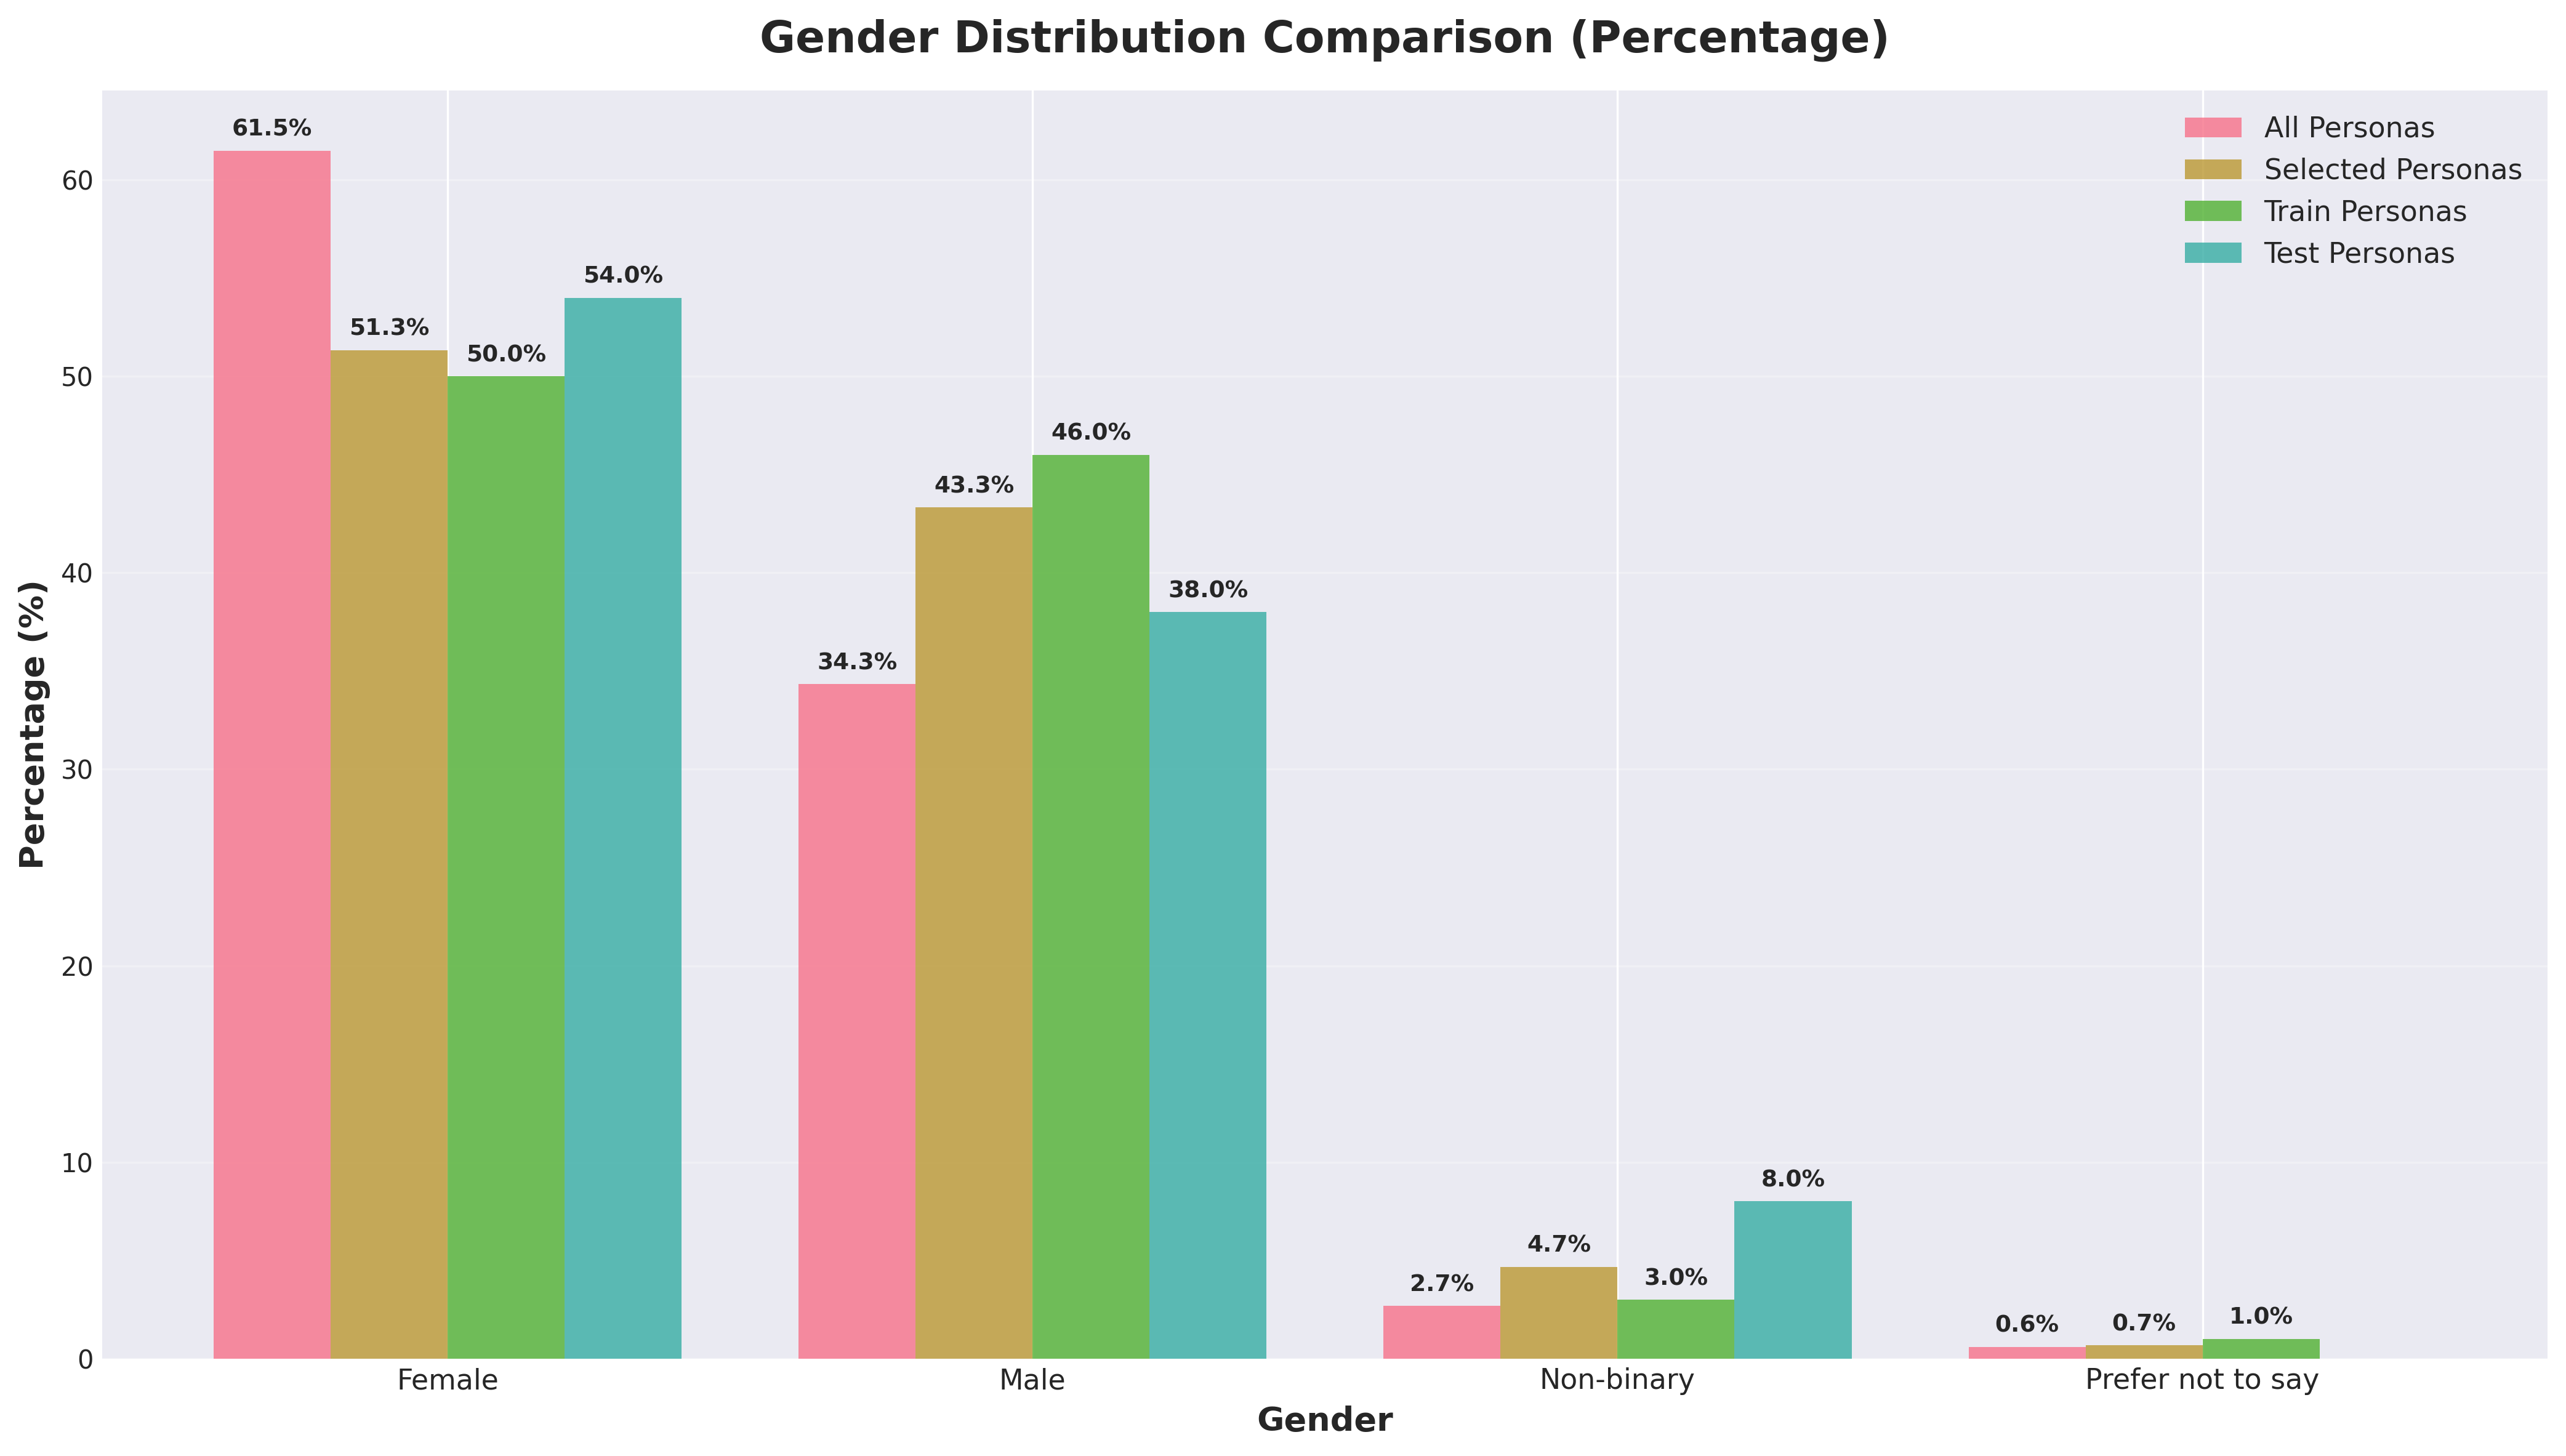}
        \caption{Gender distribution}
        \label{fig:demographics_gender}
    \end{subfigure}
    
    \begin{subfigure}[b]{0.6\textwidth}
        \centering
        \includegraphics[width=\textwidth]{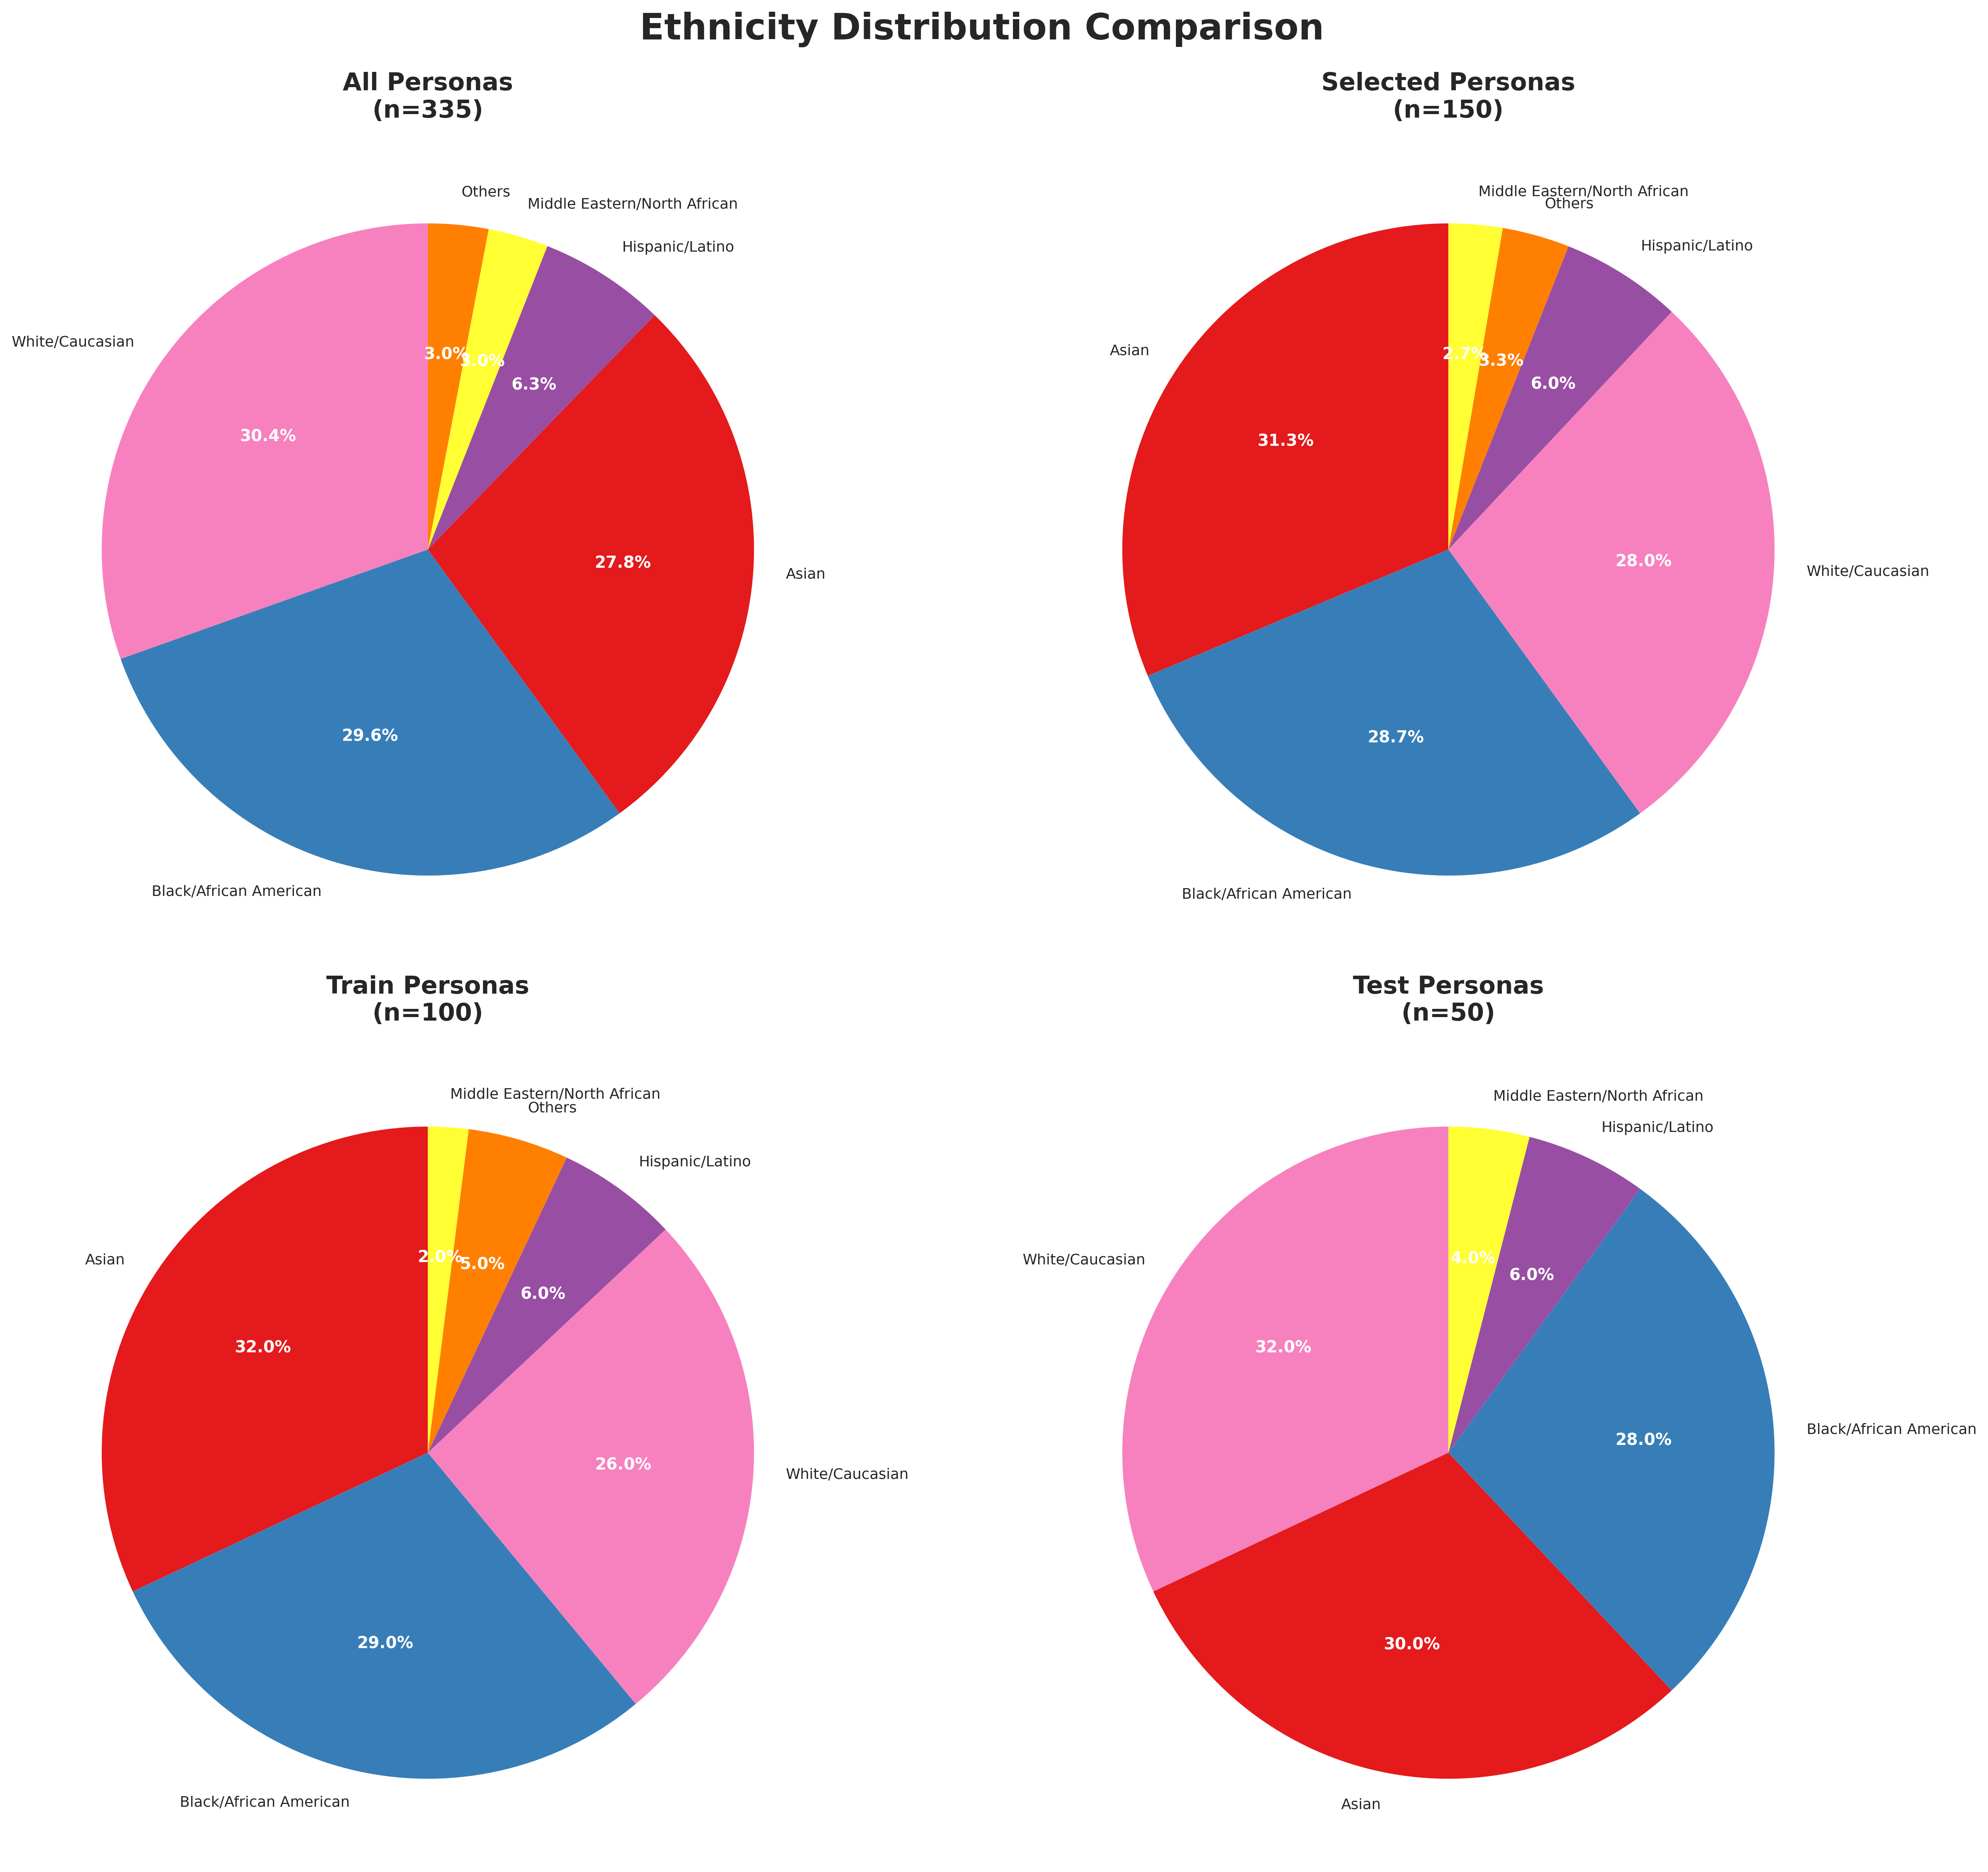}
        \caption{Ethnicity distribution}
        \label{fig:demographics_ethnicity}
    \end{subfigure}
    
    \caption{Demographic composition across complete pool (n=335), selected subset (n=150), training set (n=100), and test set (n=50).}
    \label{fig:demographics}
\end{figure}

% Figure 2: Train-test split validation
\begin{figure}[htbp]
    \centering
    \includegraphics[width=0.6\textwidth]{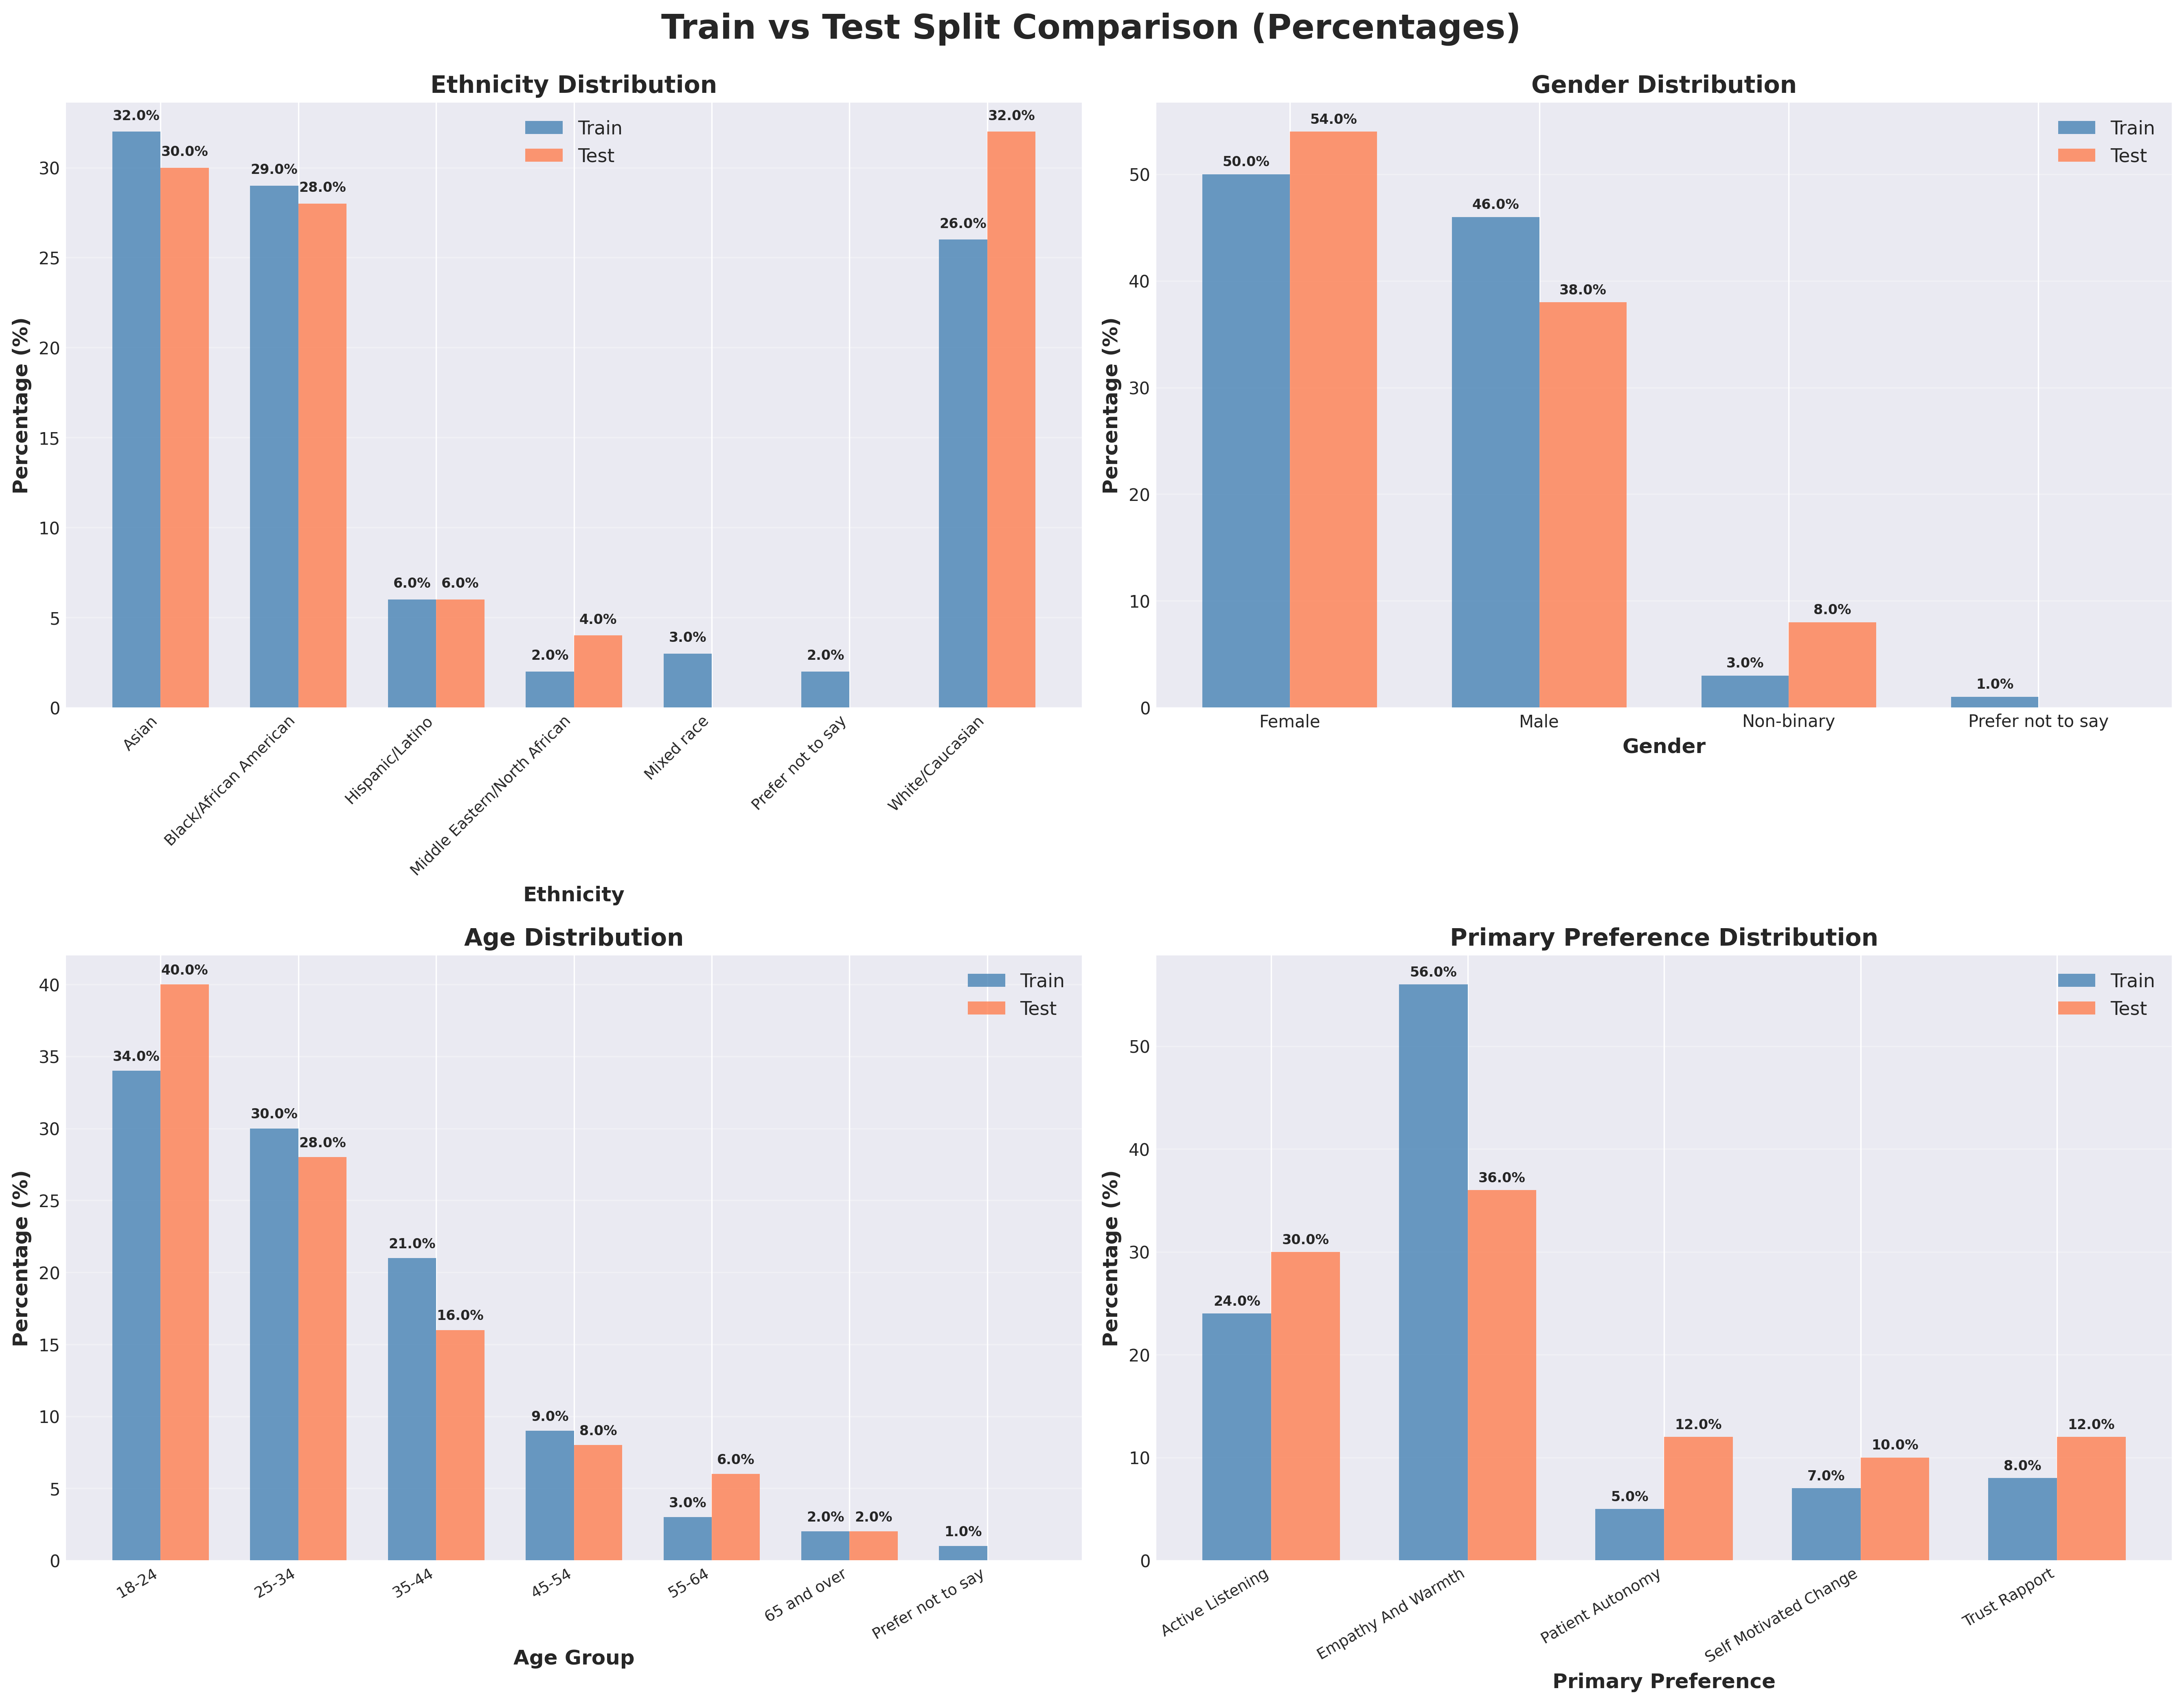}
    \caption{Train-test split demographic balance comparison.}
    \label{fig:train_test_split}
\end{figure}
\section{Training Configuration Details}
\label{appendix:training_details}

\subsection{Complete Pairwise Comparisons}
\label{appendix:pairwise_c}

Figure~\ref{fig:phase1_headtohead} presents the detailed head-to-head win rates underlying these overall rankings. Each cell shows the percentage of questions (out of 600) where the row model was preferred over the column model based on majority voting among the 50 patient personas.

\begin{figure}[htbp]
    \centering
    \begin{subfigure}[b]{0.48\textwidth}
        \centering
        \includegraphics[width=\textwidth]{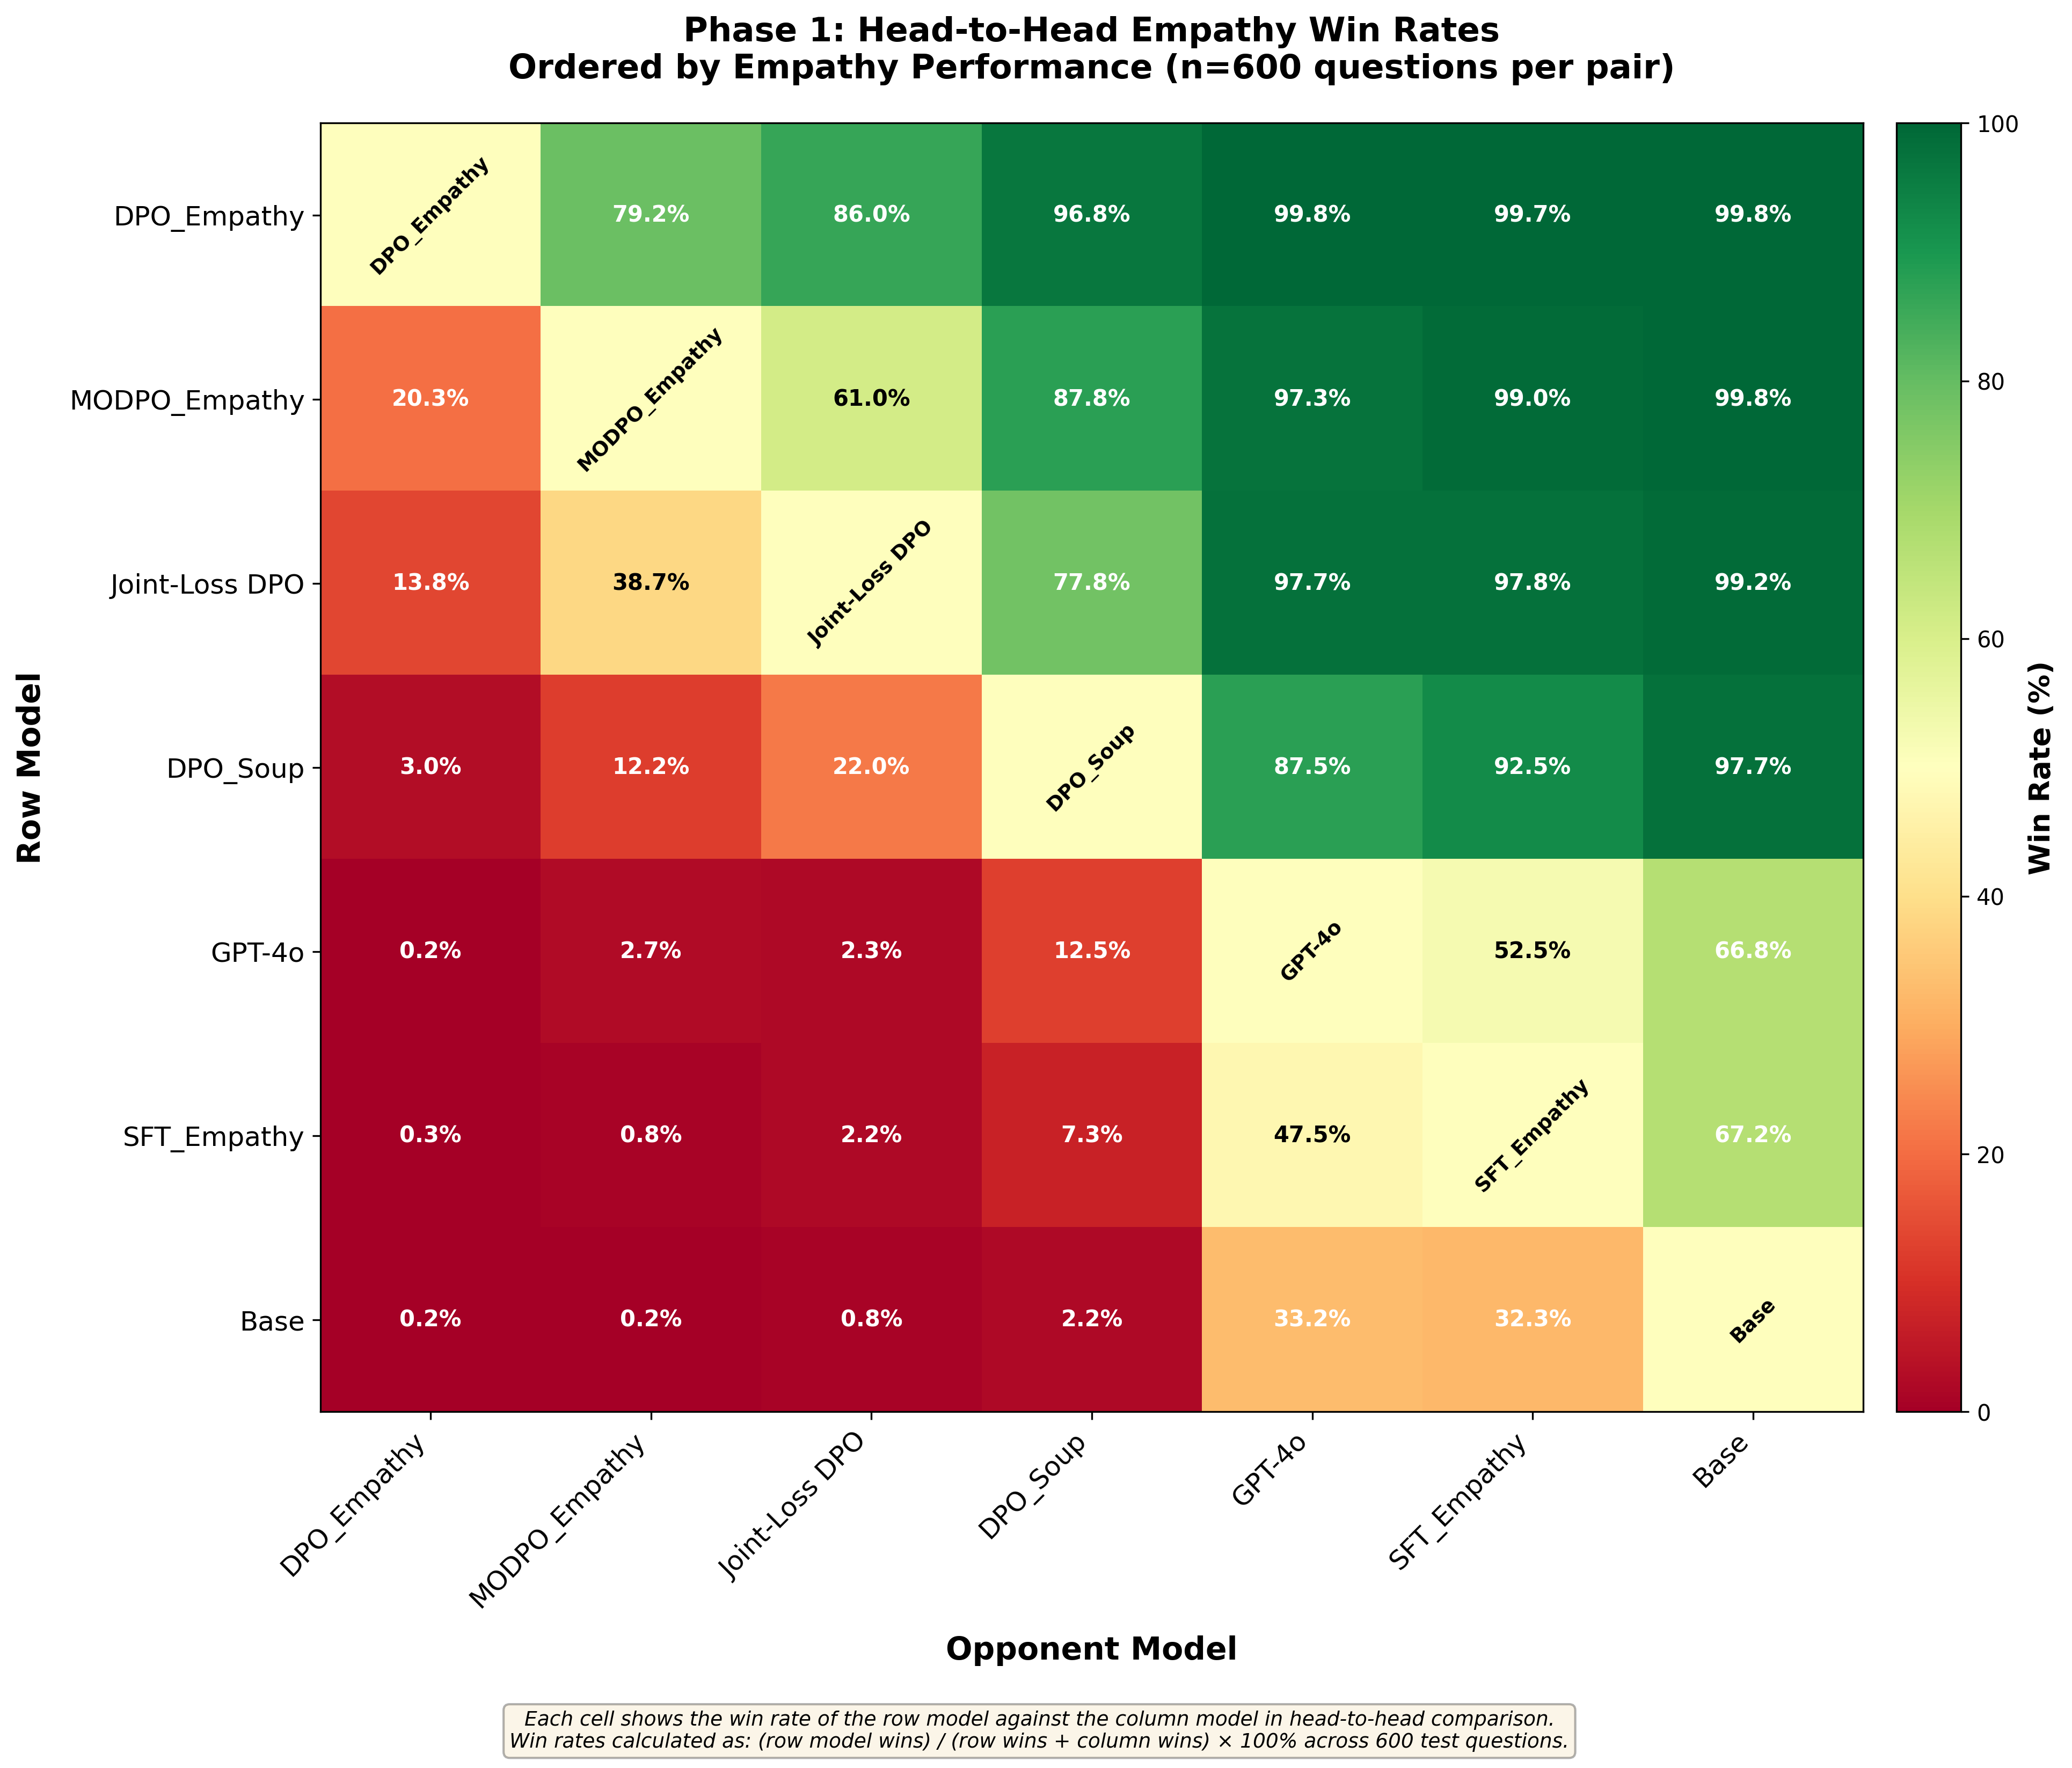}
        \caption{Empathy pairwise win rates}
        \label{fig:phase1_headtohead_empathy}
    \end{subfigure}
    \hfill
    \begin{subfigure}[b]{0.48\textwidth}
        \centering
        \includegraphics[width=\textwidth]{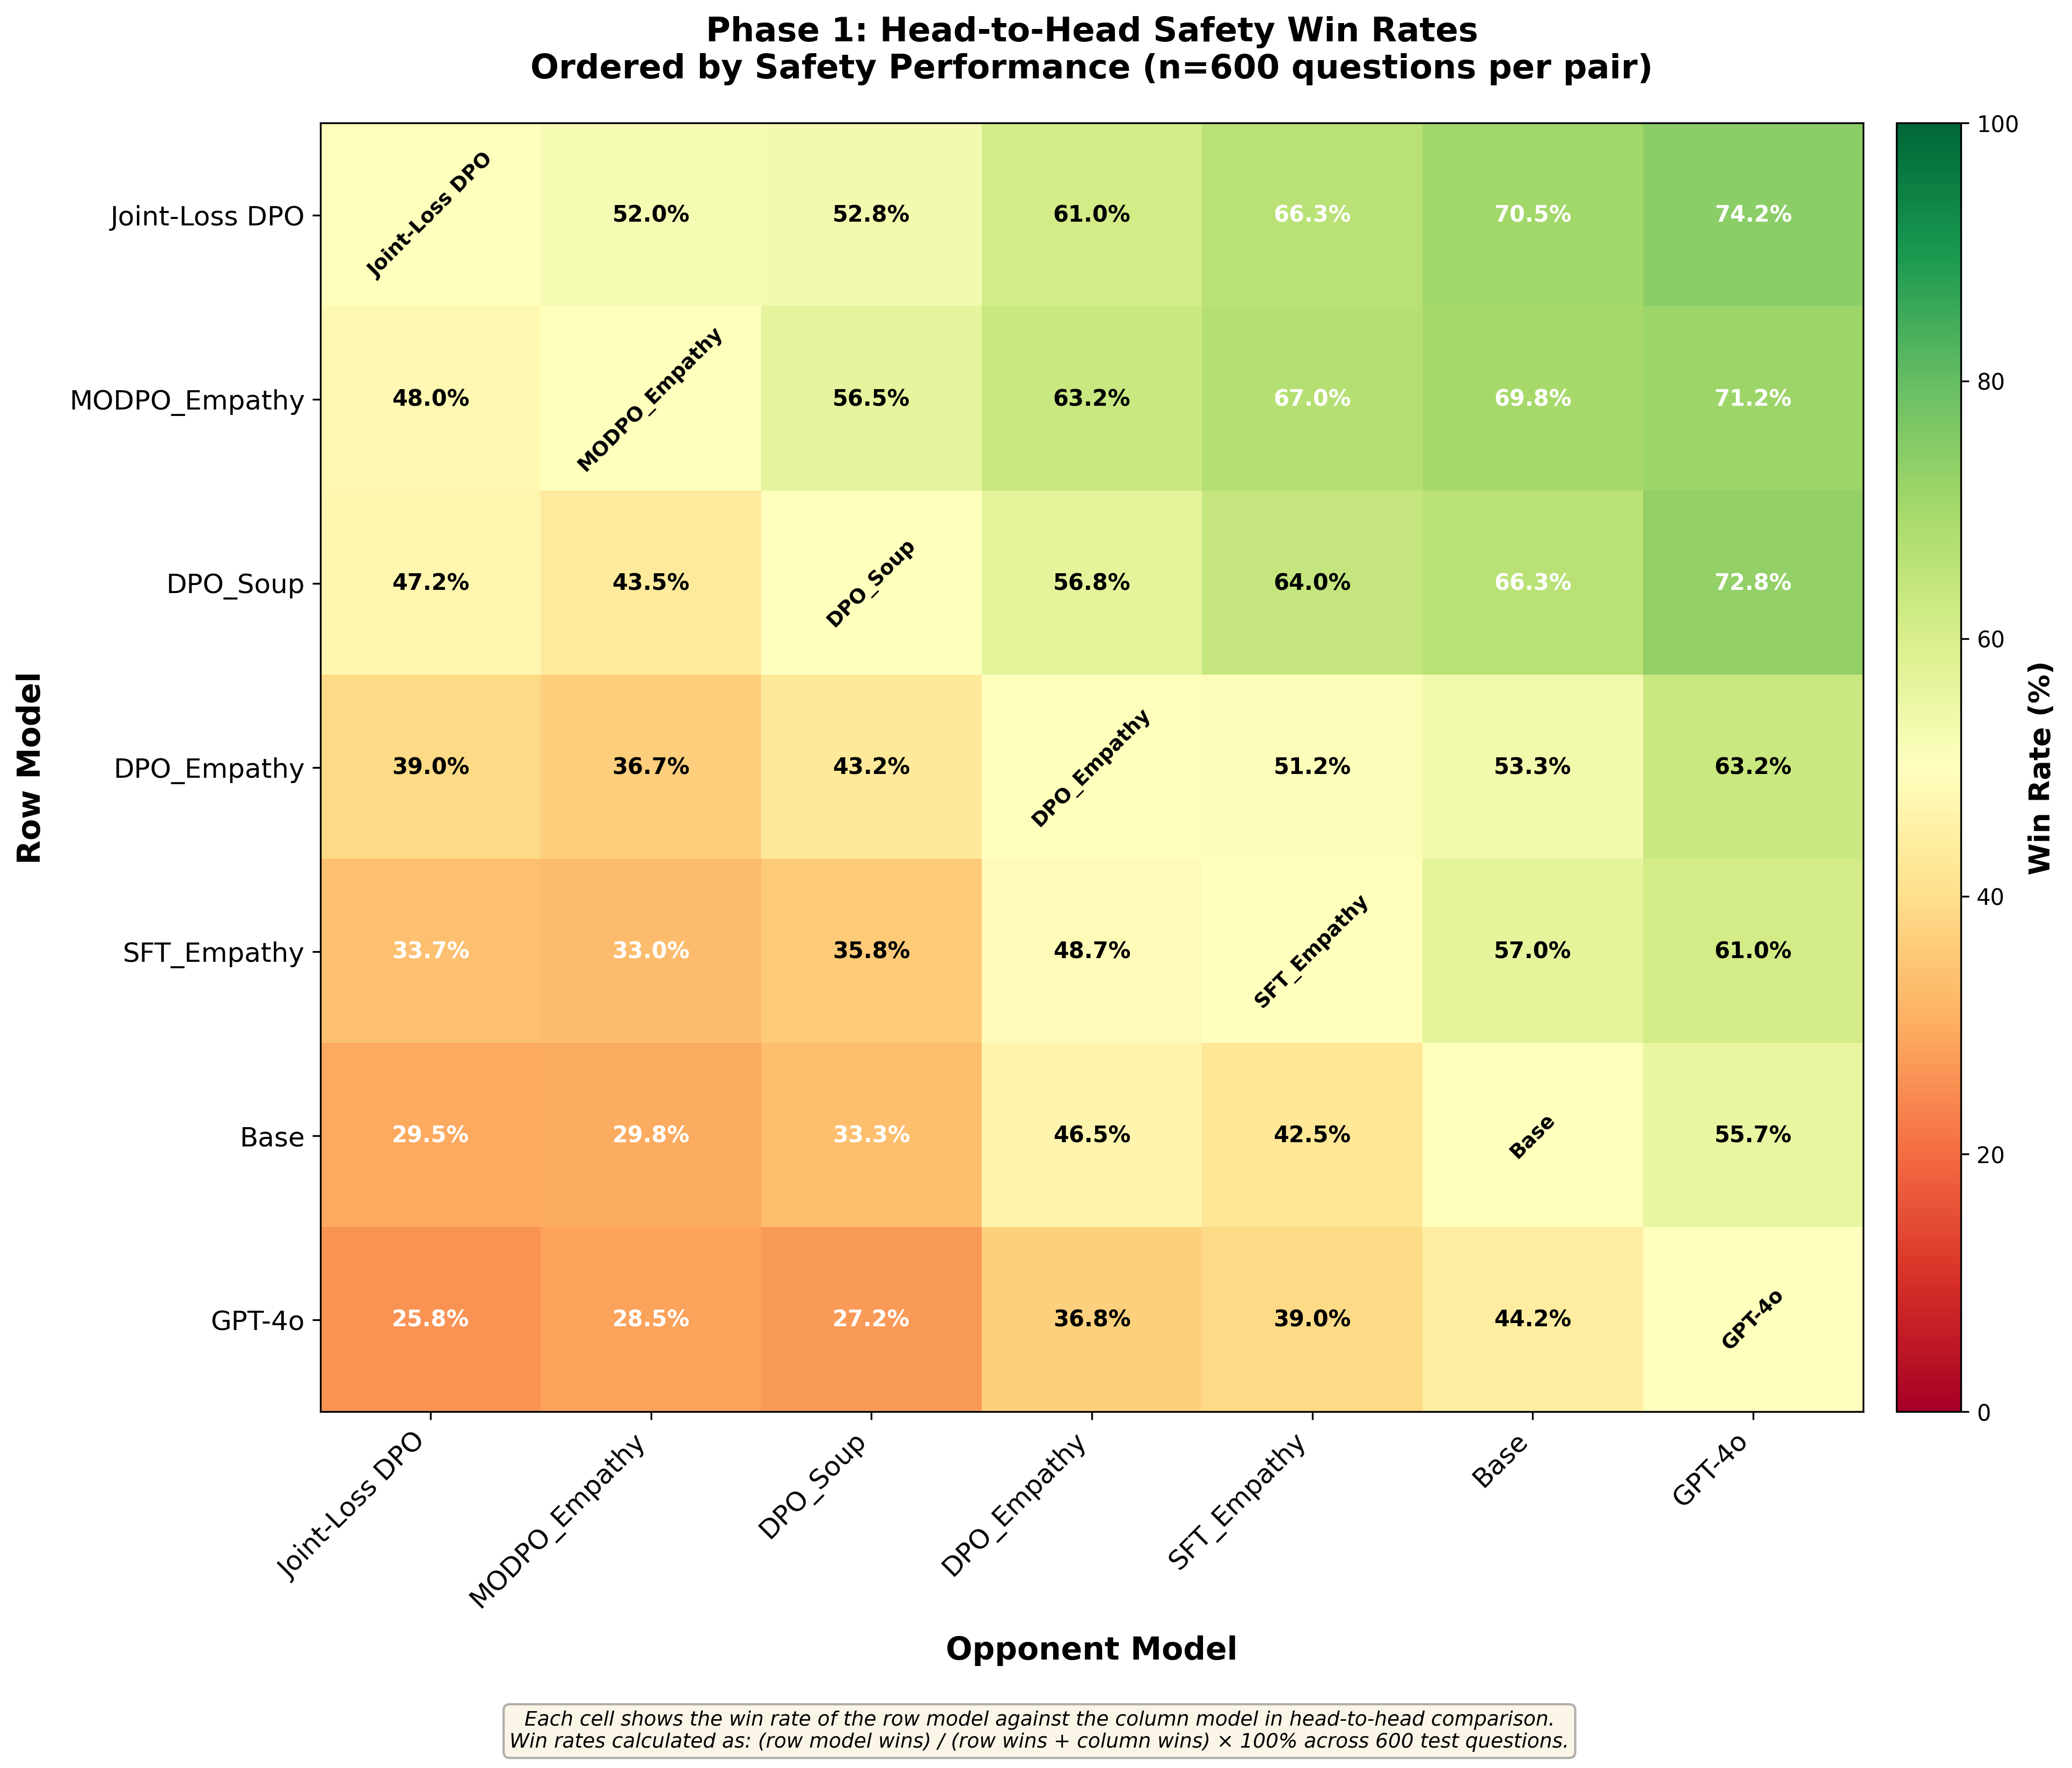}
        \caption{Safety pairwise win rates}
        \label{fig:phase1_headtohead_safety}
    \end{subfigure}
    \caption{Complete head-to-head win rates for all 21 pairwise comparisons. Each cell displays the row model's win rate against the column model. Models ordered by performance (best to worst) within each dimension.}
    \label{fig:phase1_headtohead}
\end{figure}

On empathy, DPO\_Empathy achieved near-perfect dominance, winning 99.8\% against Base and GPT-4o, 96.8\% against DPO\_Soup, and 79-86\% against the multi-objective methods. MODPO\_Empathy demonstrated strong second-tier performance with 87.8\% against DPO\_Soup and 97.3-99.8\% against lower-performing models. Joint-Loss DPO showed intermediate strength, defeating DPO\_Soup by 77.8\% but losing to MODPO by 61.0\%.

Safety comparisons revealed more competitive matchups. MODPO\_Empathy and Joint-Loss DPO traded narrow victories (52.0\% vs 48.0\%), confirming their near-tie. Both beat DPO\_Soup (56.5\% and 52.8\% respectively), who in turn beat DPO\_Empathy (56.8\%). The baseline models showed consistently poor performance, with GPT-4o achieving win rates below 40\% against all trained models.

\subsection{Phase 2 Additional Results}

Figure~\ref{fig:phase2_winrates} displays dimension-specific rankings.

\begin{figure}[htbp]
    \centering
    \begin{subfigure}[b]{0.48\textwidth}
        \centering
        \includegraphics[width=\textwidth]{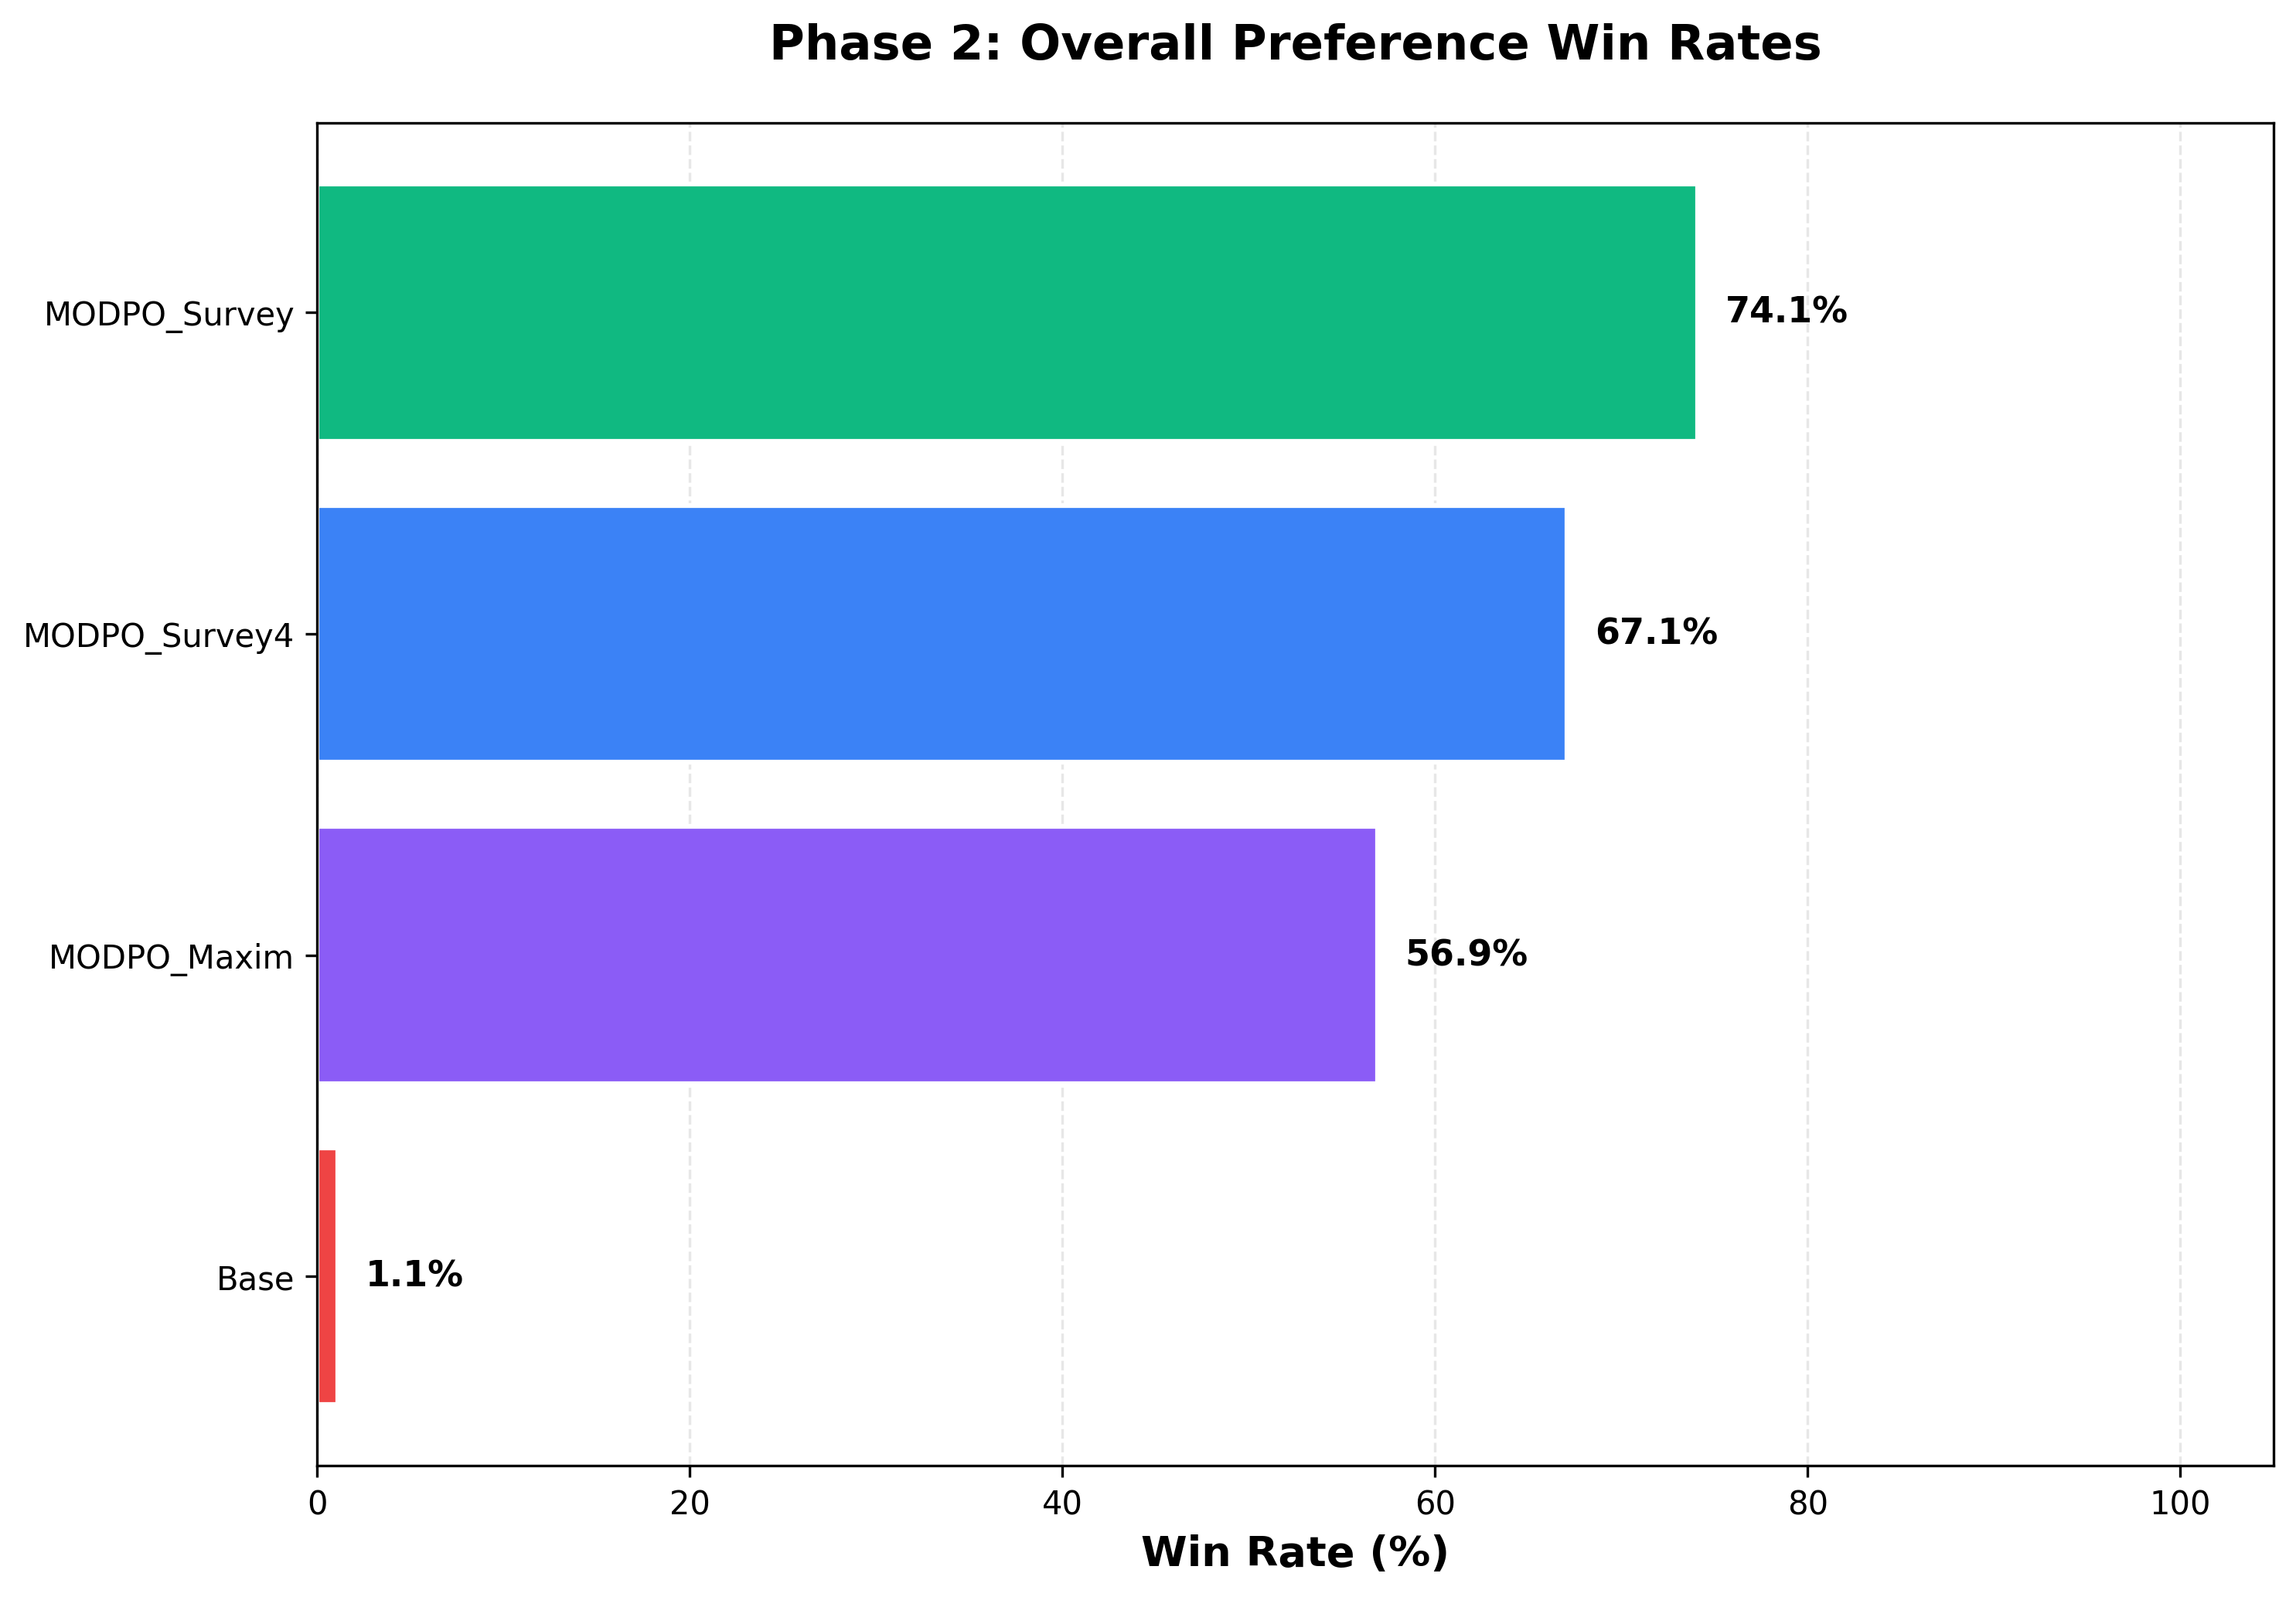}
        \caption{Overall Preference}
    \end{subfigure}
    \hfill
    \begin{subfigure}[b]{0.48\textwidth}
        \centering
        \includegraphics[width=\textwidth]{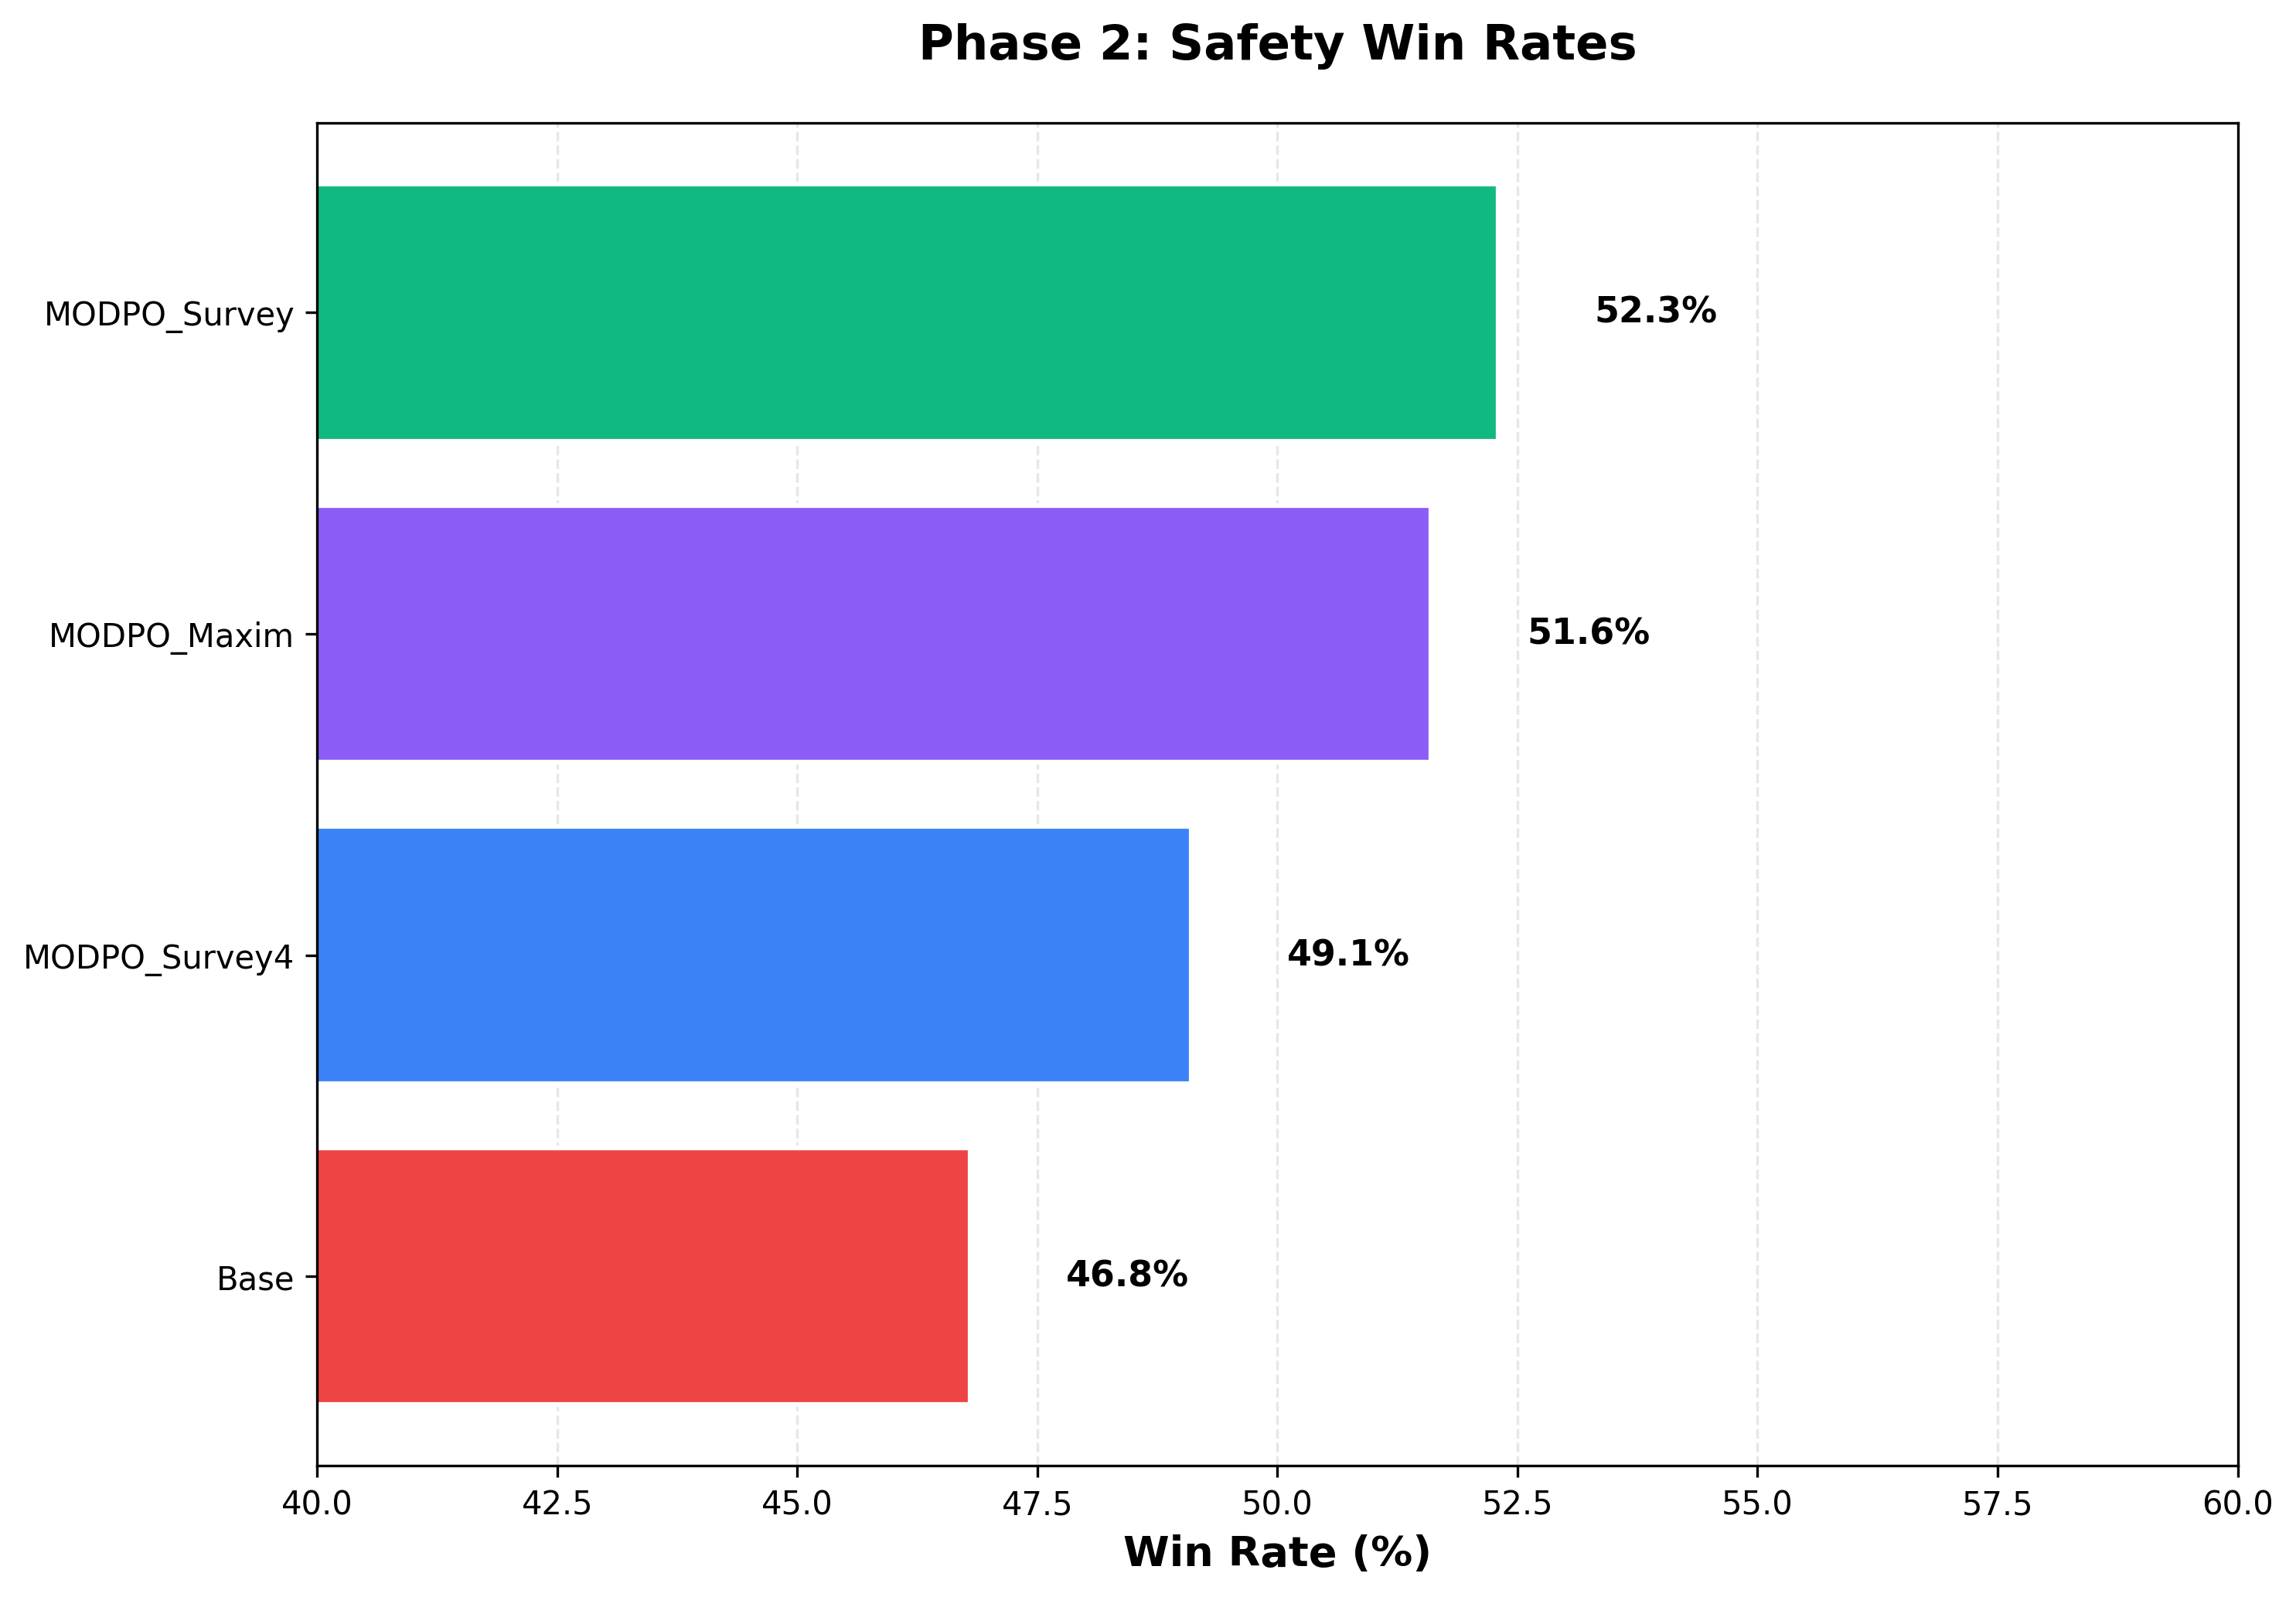}
        \caption{Safety}
    \end{subfigure}
    \caption{Phase 2 performance rankings calculated as average win rate across all pairwise comparisons.}
    \label{fig:phase2_winrates}
\end{figure}

\subsubsection{Head-to-Head Comparisons}

Figure~\ref{fig:phase2_headtohead} presents detailed pairwise win rates underlying these rankings. Each cell shows the percentage of questions (out of 600) where the row model was preferred over the column model.

\begin{figure}[htbp]
    \centering
    \begin{subfigure}[b]{0.48\textwidth}
        \centering
        \includegraphics[width=\textwidth]{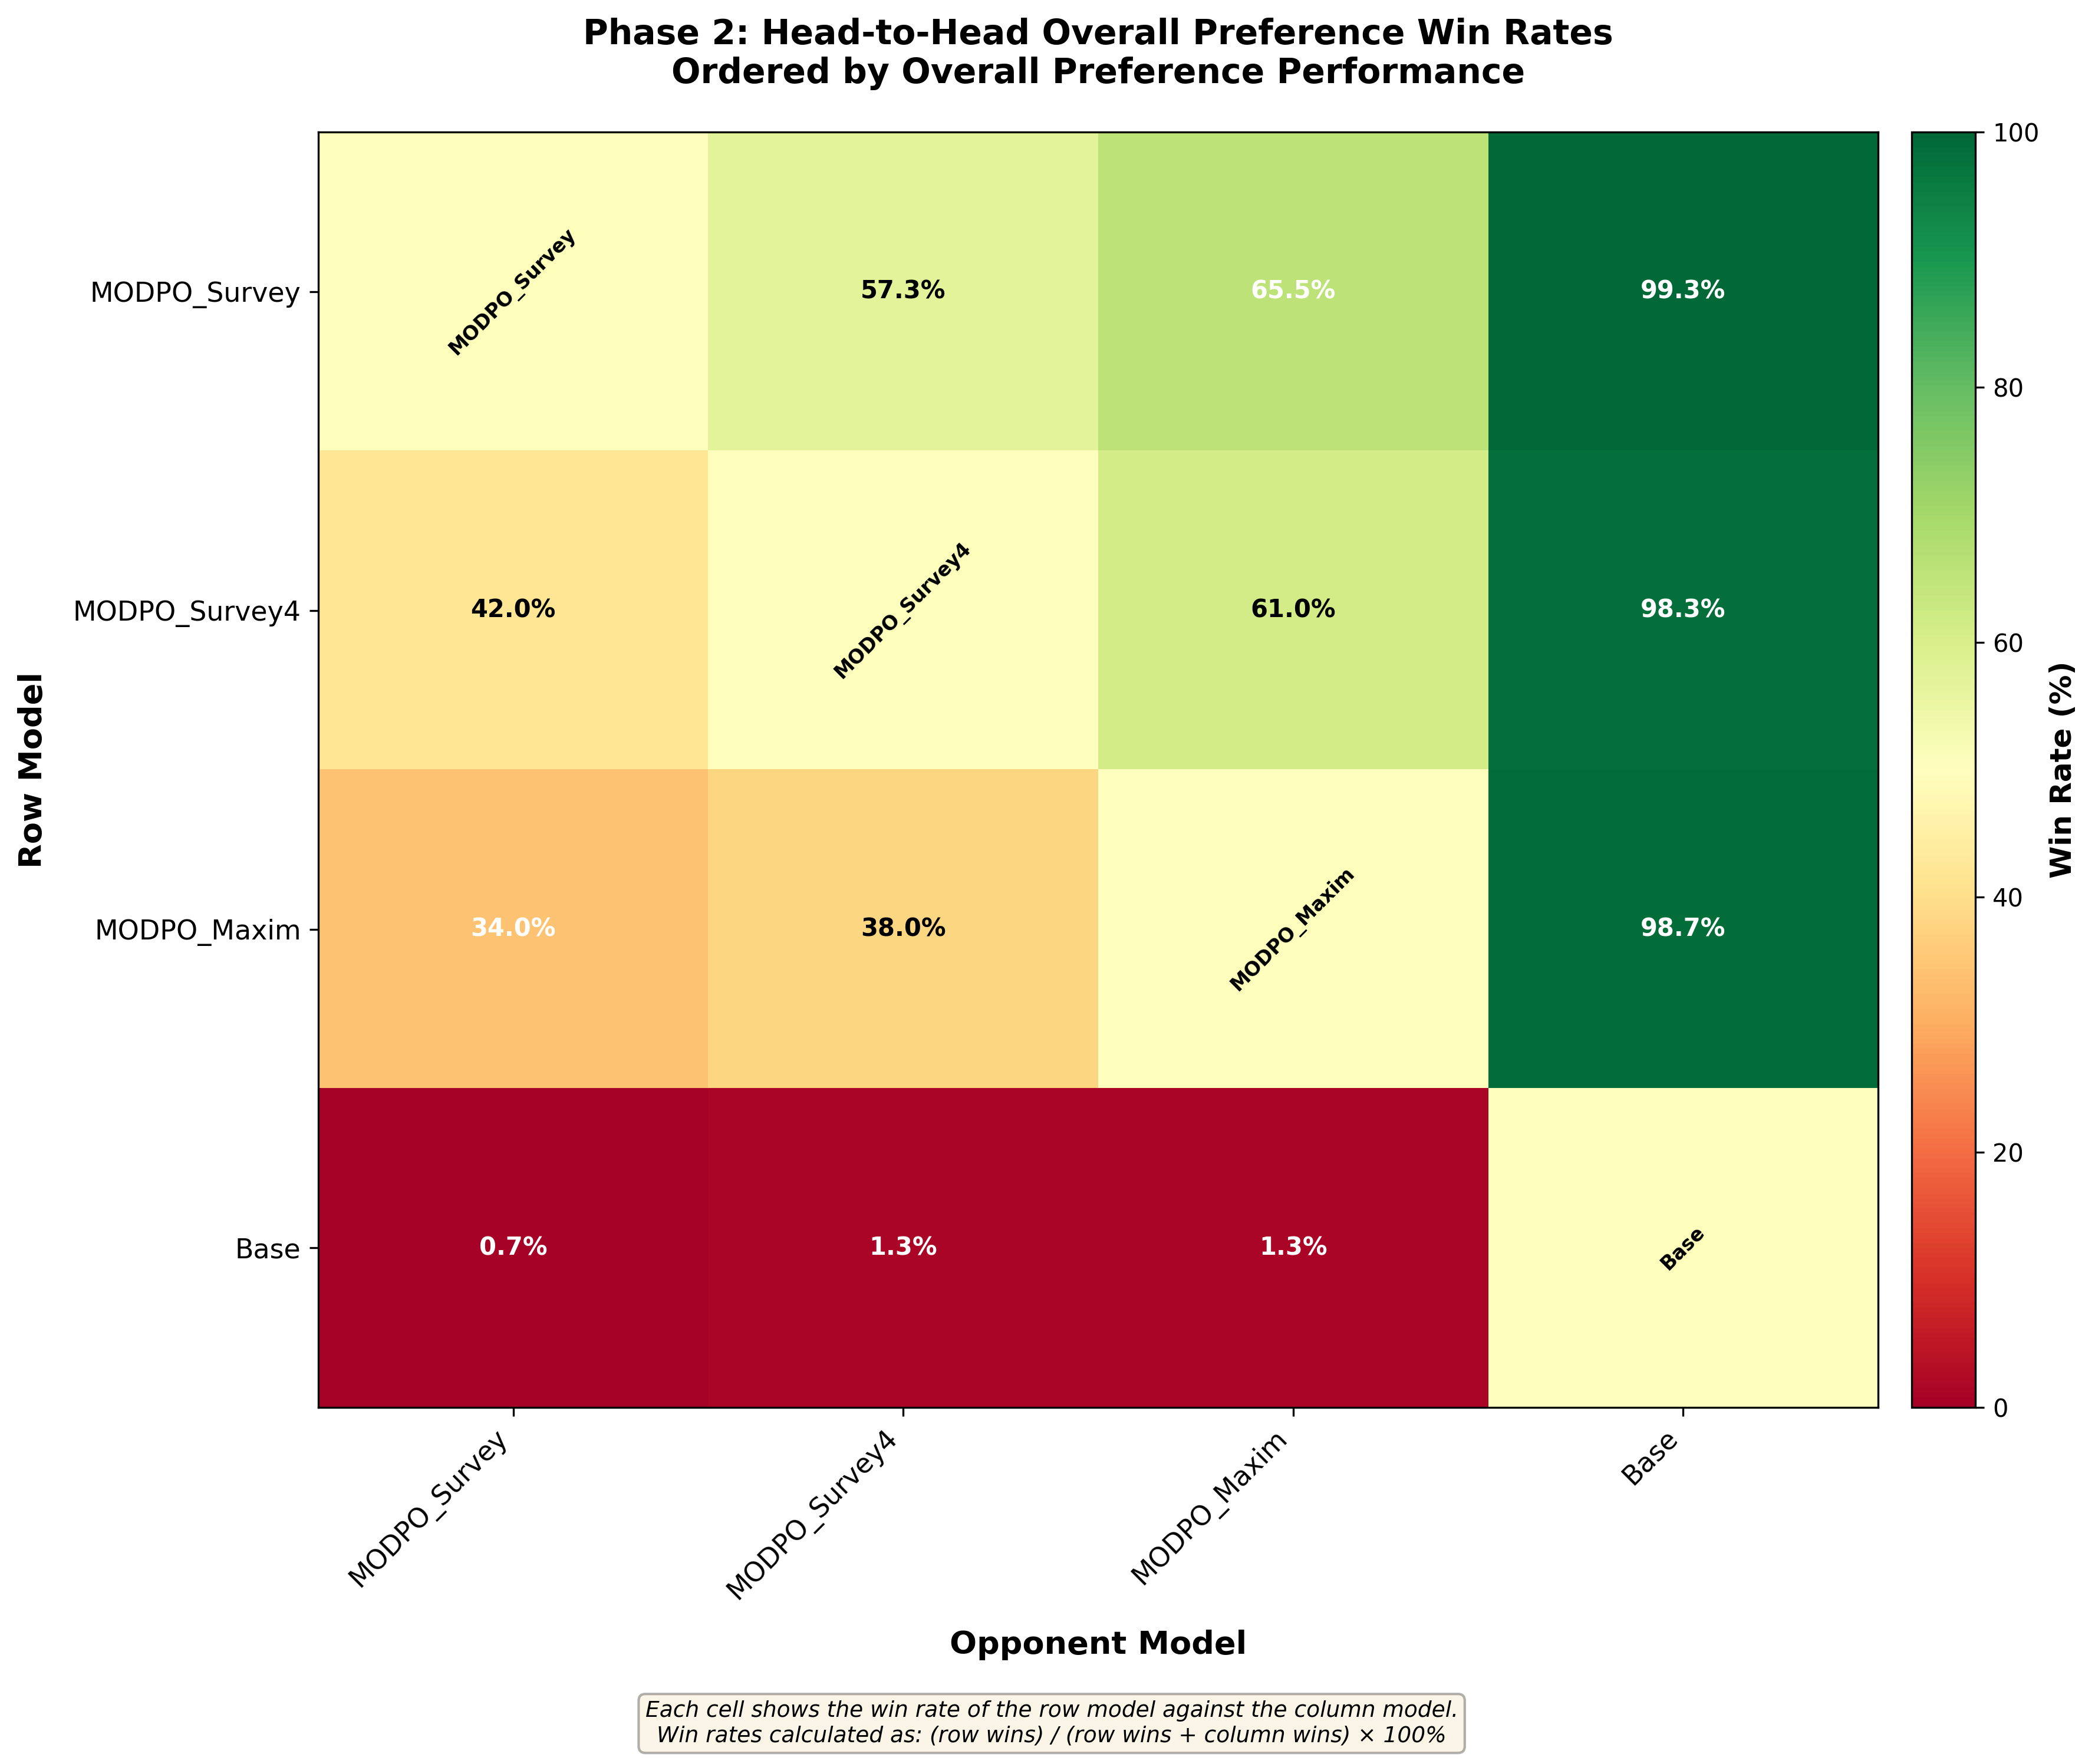}
        \caption{Overall Preference}
        \label{fig:phase2_headtohead_overall}
    \end{subfigure}
    \hfill
    \begin{subfigure}[b]{0.48\textwidth}
        \centering
        \includegraphics[width=\textwidth]{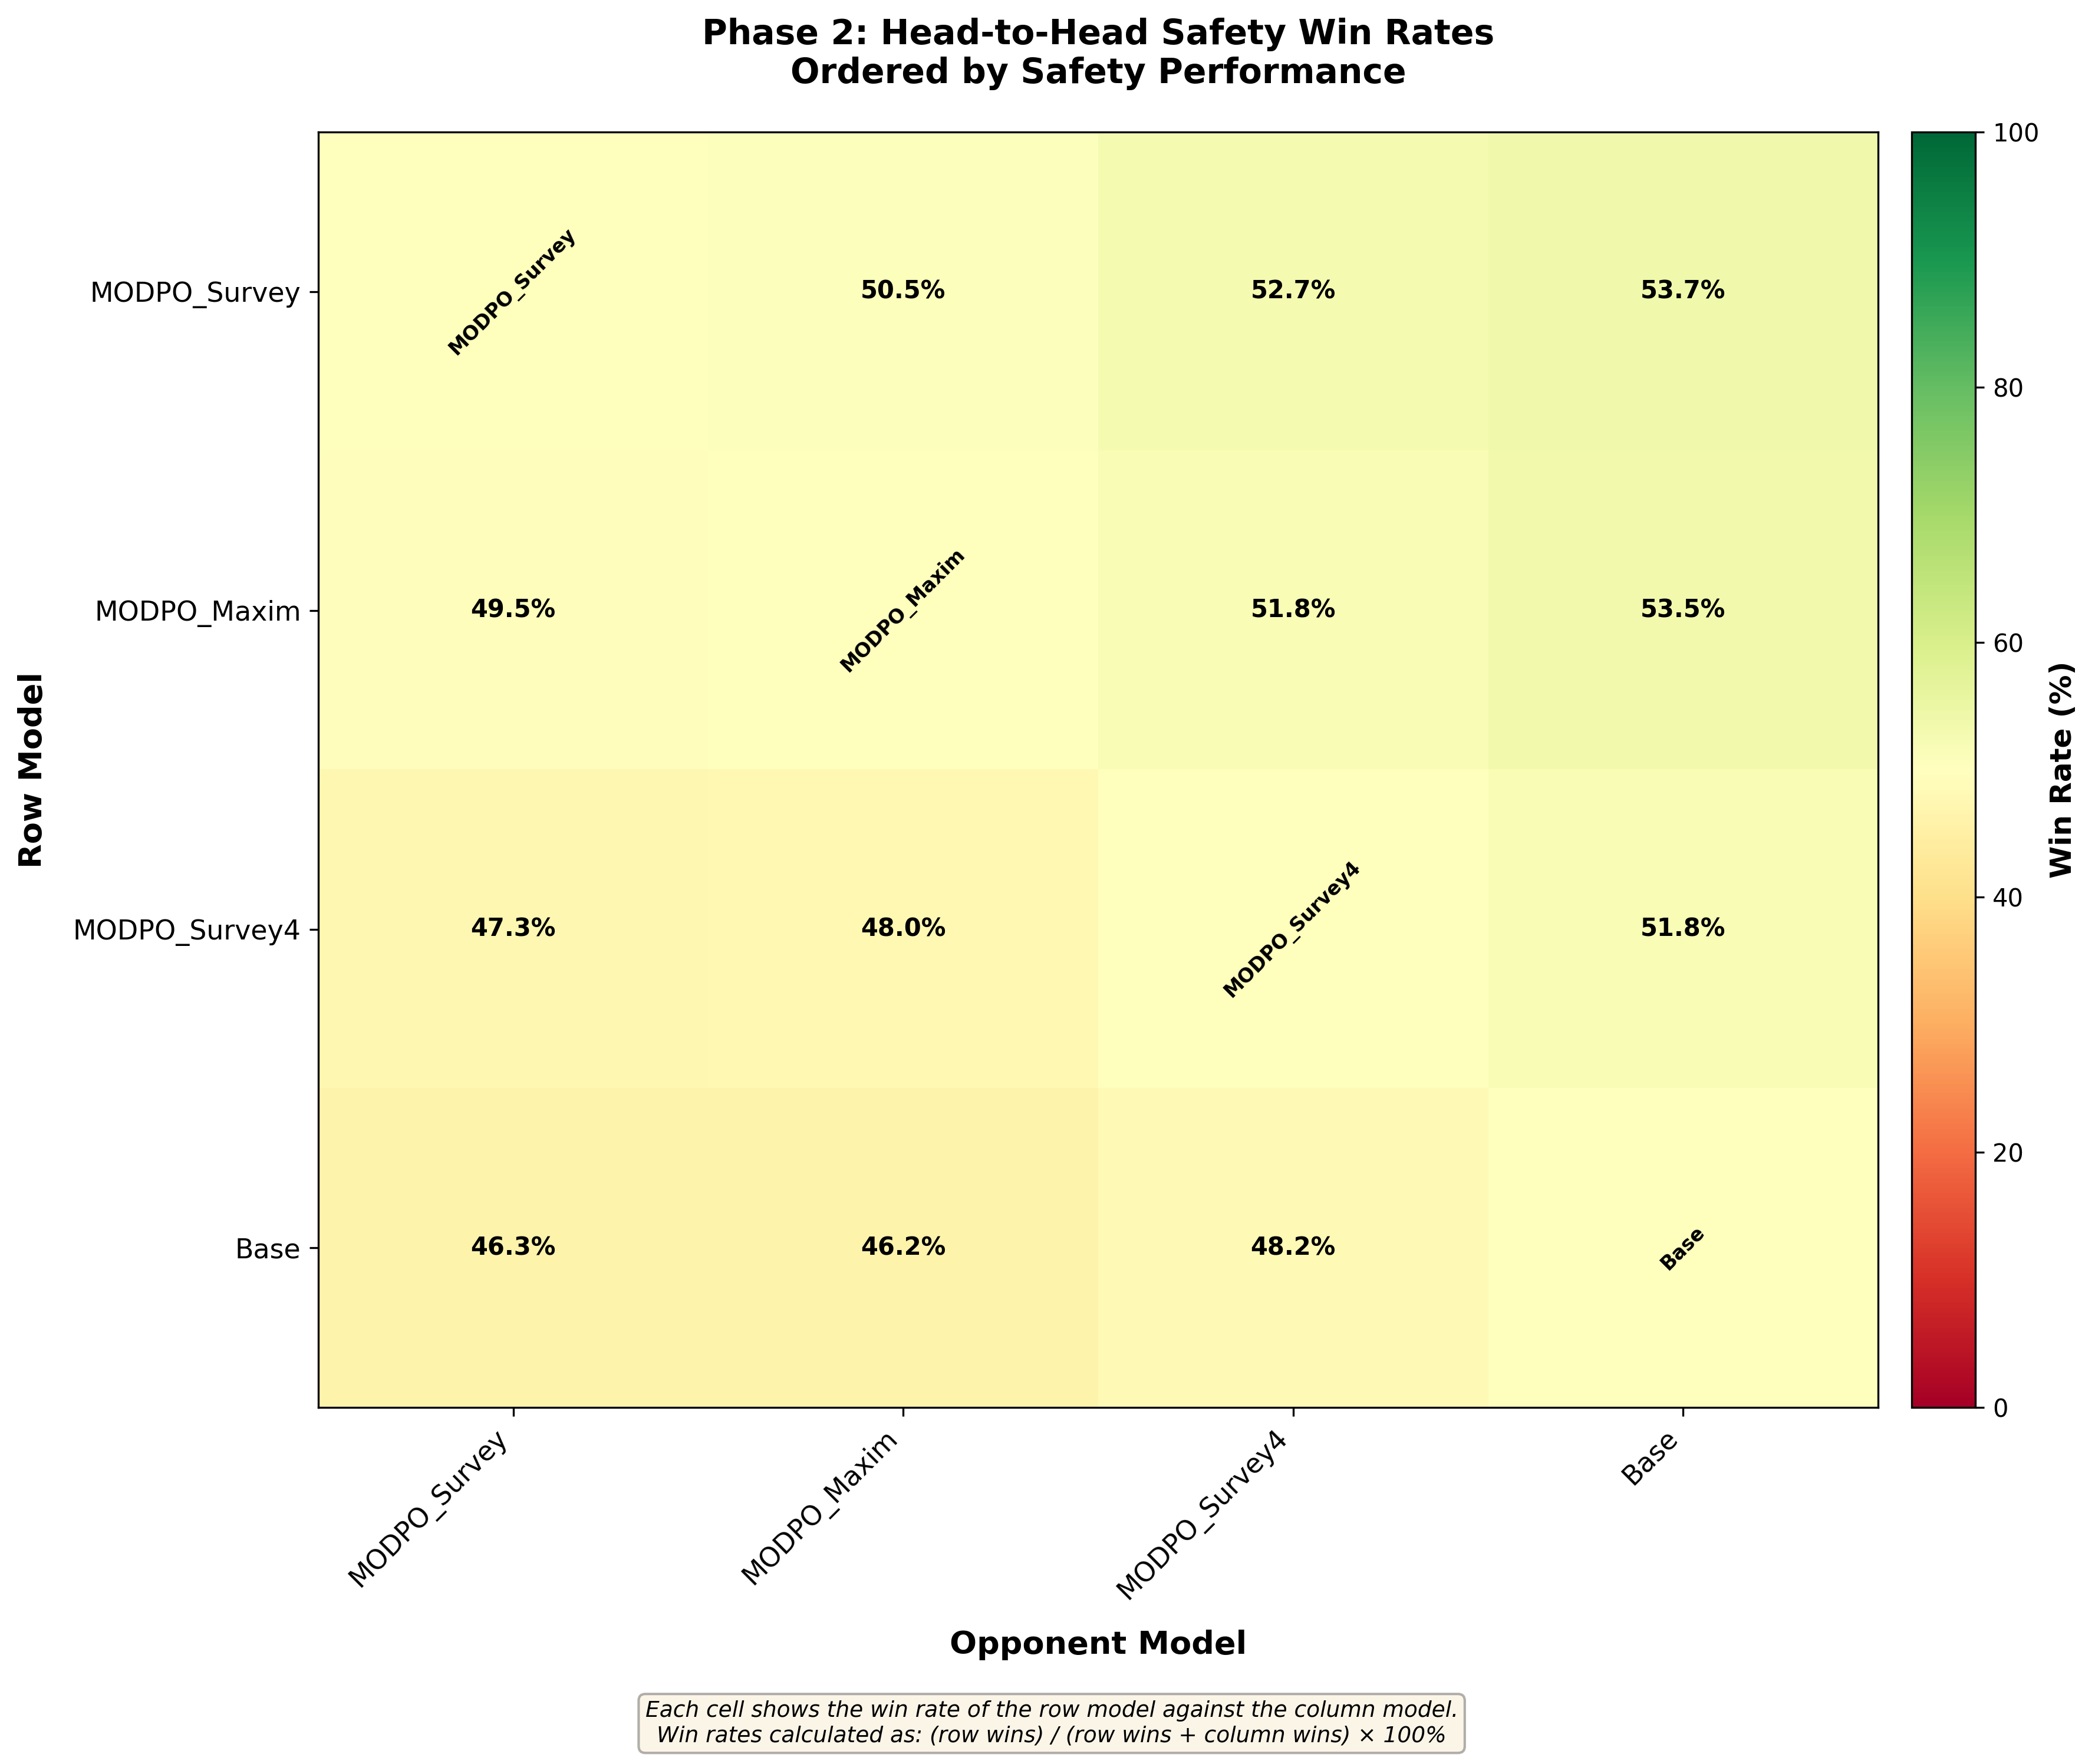}
        \caption{Safety}
        \label{fig:phase2_headtohead_safety}
    \end{subfigure}
    \caption{Complete head-to-head win rates for all pairwise comparisons. Models ordered by performance within each dimension.}
    \label{fig:phase2_headtohead}
\end{figure}

Overall preference comparisons revealed decisive advantages for therapeutic-specific criteria. MODPO\_Survey achieved strong victories over all competitors: 65.5\% against MODPO\_Maxim, 57.3\% against MODPO\_Survey4, and 99.3\% against Base. MODPO\_Survey4 similarly outperformed MODPO\_Maxim (61.0\%) and Base (98.3\%). These results confirm that therapeutic-specific criteria (Survey, Survey4) consistently produce responses patients prefer over general communication principles (Maxim), with margins of 23-31.5 percentage points in direct comparisons.

Safety comparisons showed more balanced results among trained models. MODPO\_Survey narrowly edged MODPO\_Maxim (50.5\%) and MODPO\_Survey4 (52.7\%), while MODPO\_Maxim achieved 51.8\% against MODPO\_Survey4. All three trained models outperformed Base: MODPO\_Survey (53.7\%), MODPO\_Maxim (53.5\%), and MODPO\_Survey4 (51.8\%).

\subsubsection{Statistical Significance}

We validated performance differences using McNemar's test on all pairwise comparisons (Figure~\ref{fig:phase2_significance}).

\begin{figure}[htbp]
    \centering
    \begin{subfigure}[b]{0.48\textwidth}
        \centering
        \includegraphics[width=\textwidth]{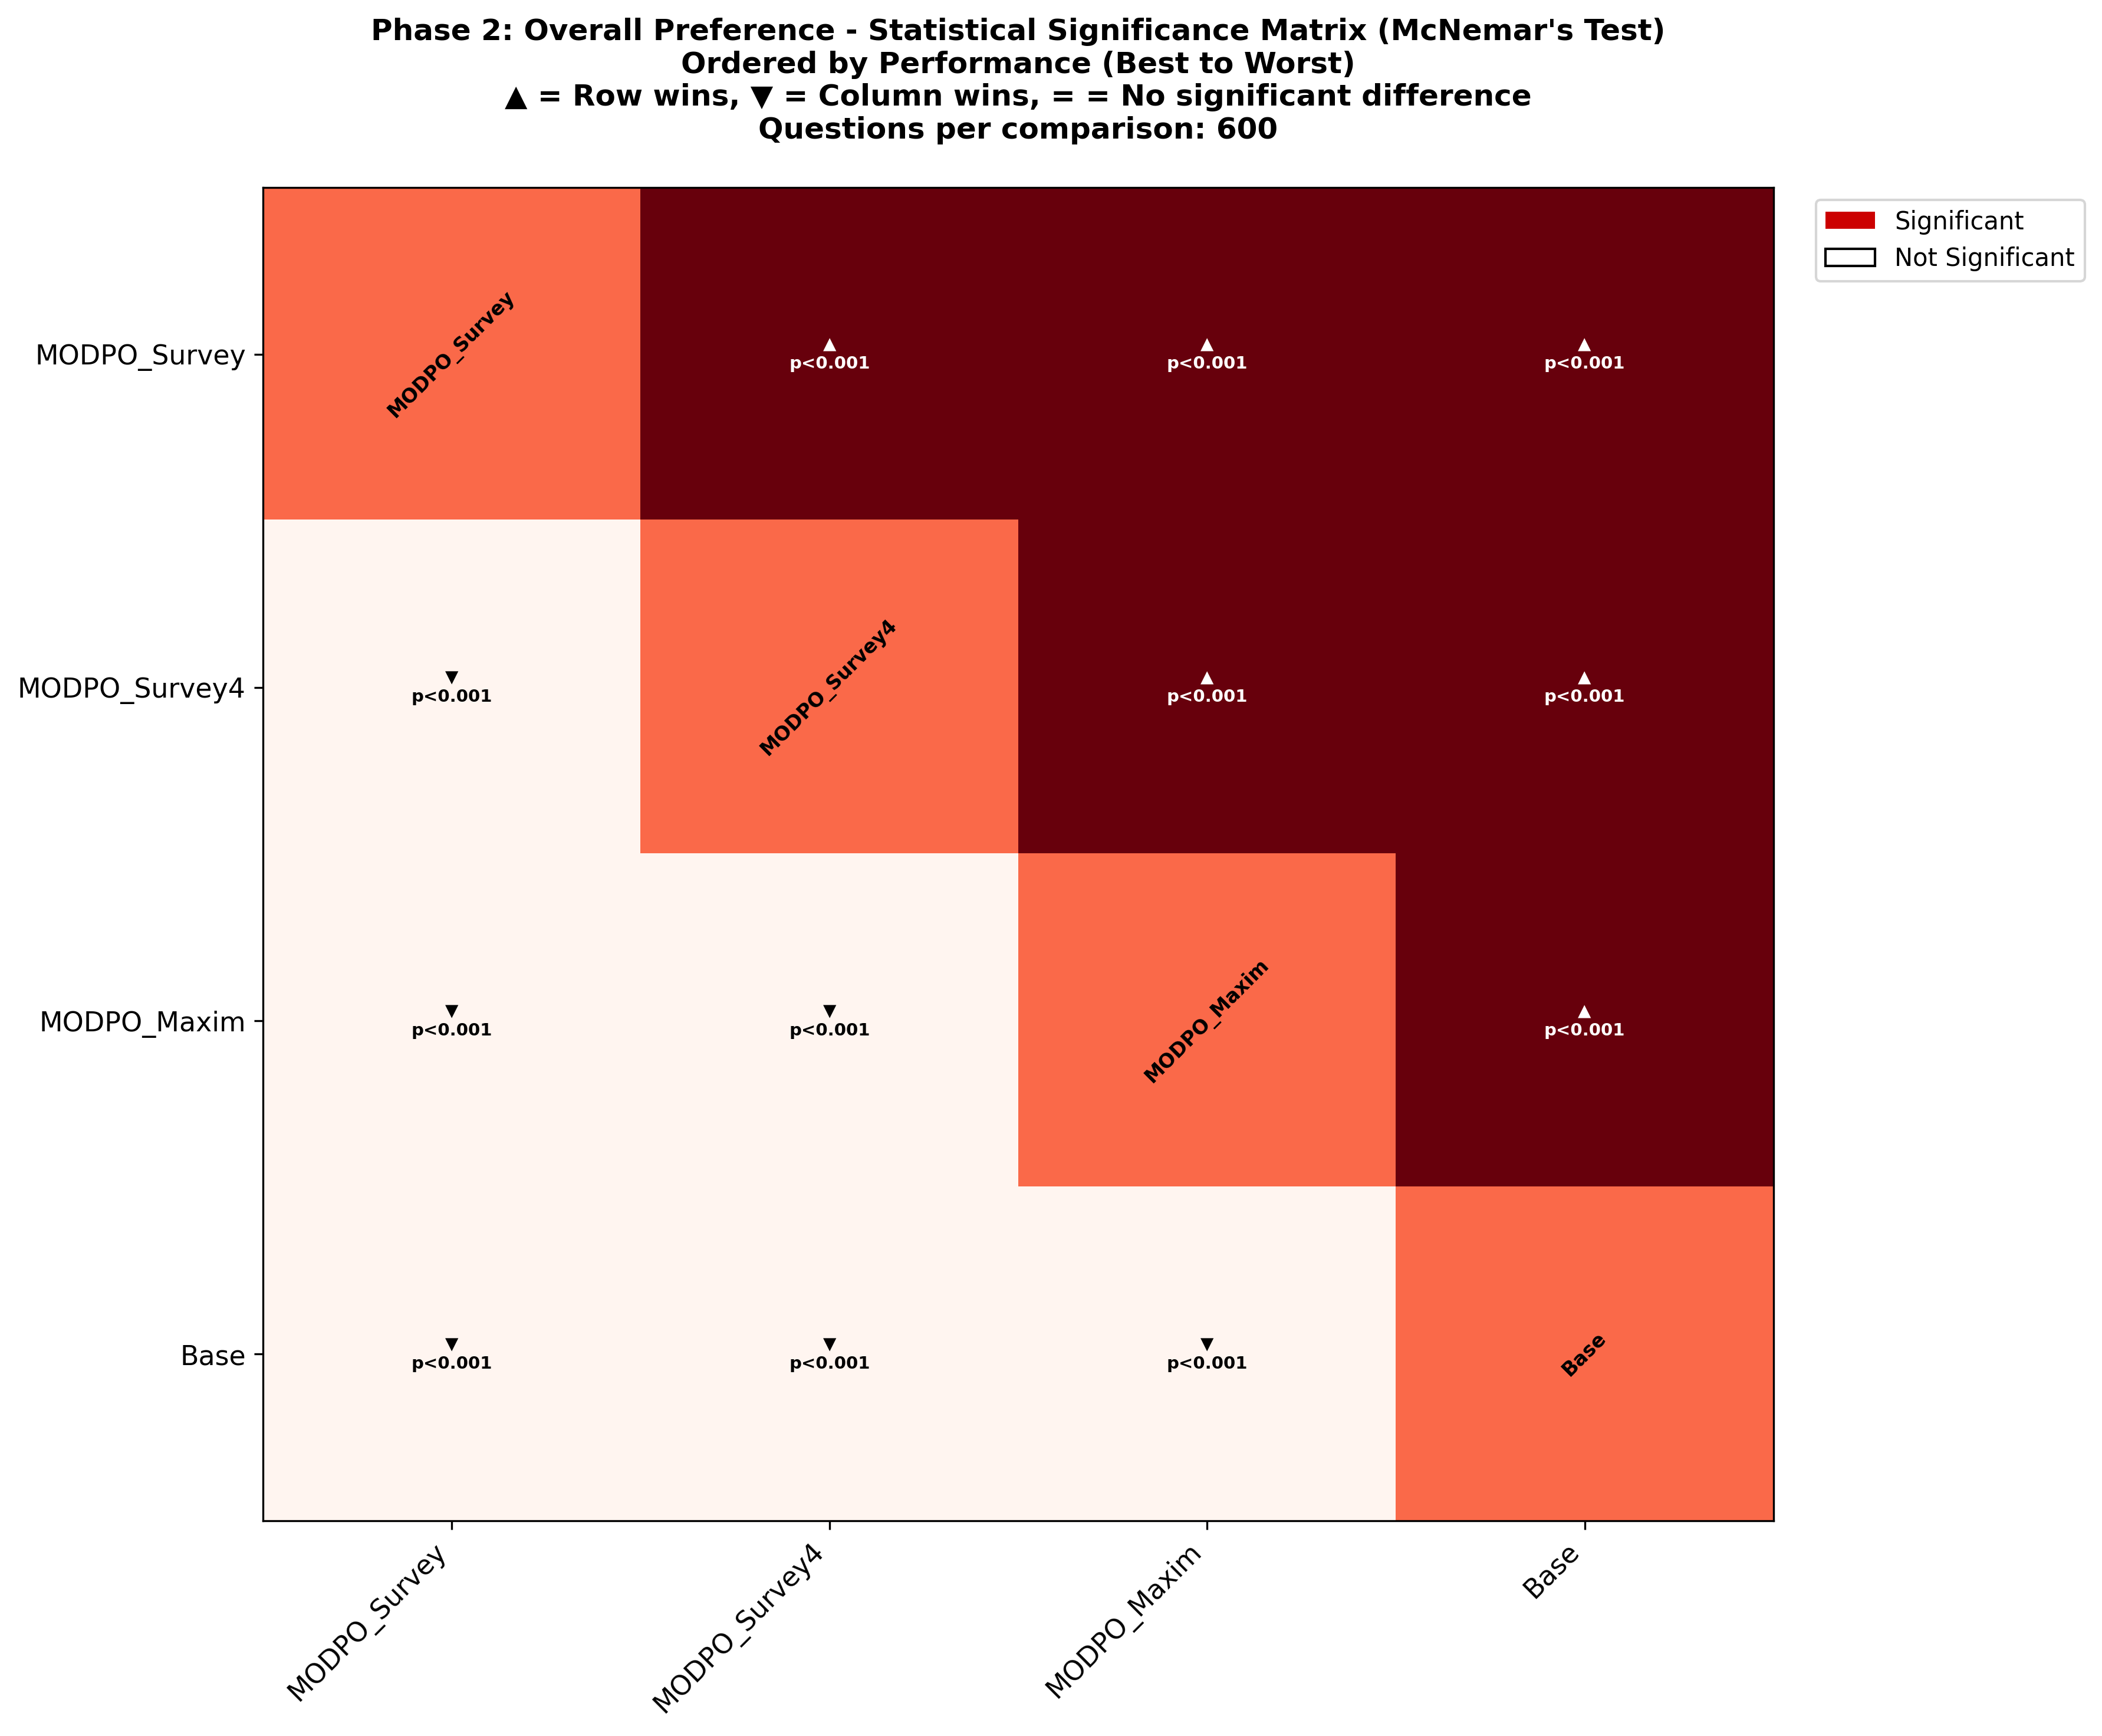}
        \caption{Overall Preference}
    \end{subfigure}
    \hfill
    \begin{subfigure}[b]{0.48\textwidth}
        \centering
        \includegraphics[width=\textwidth]{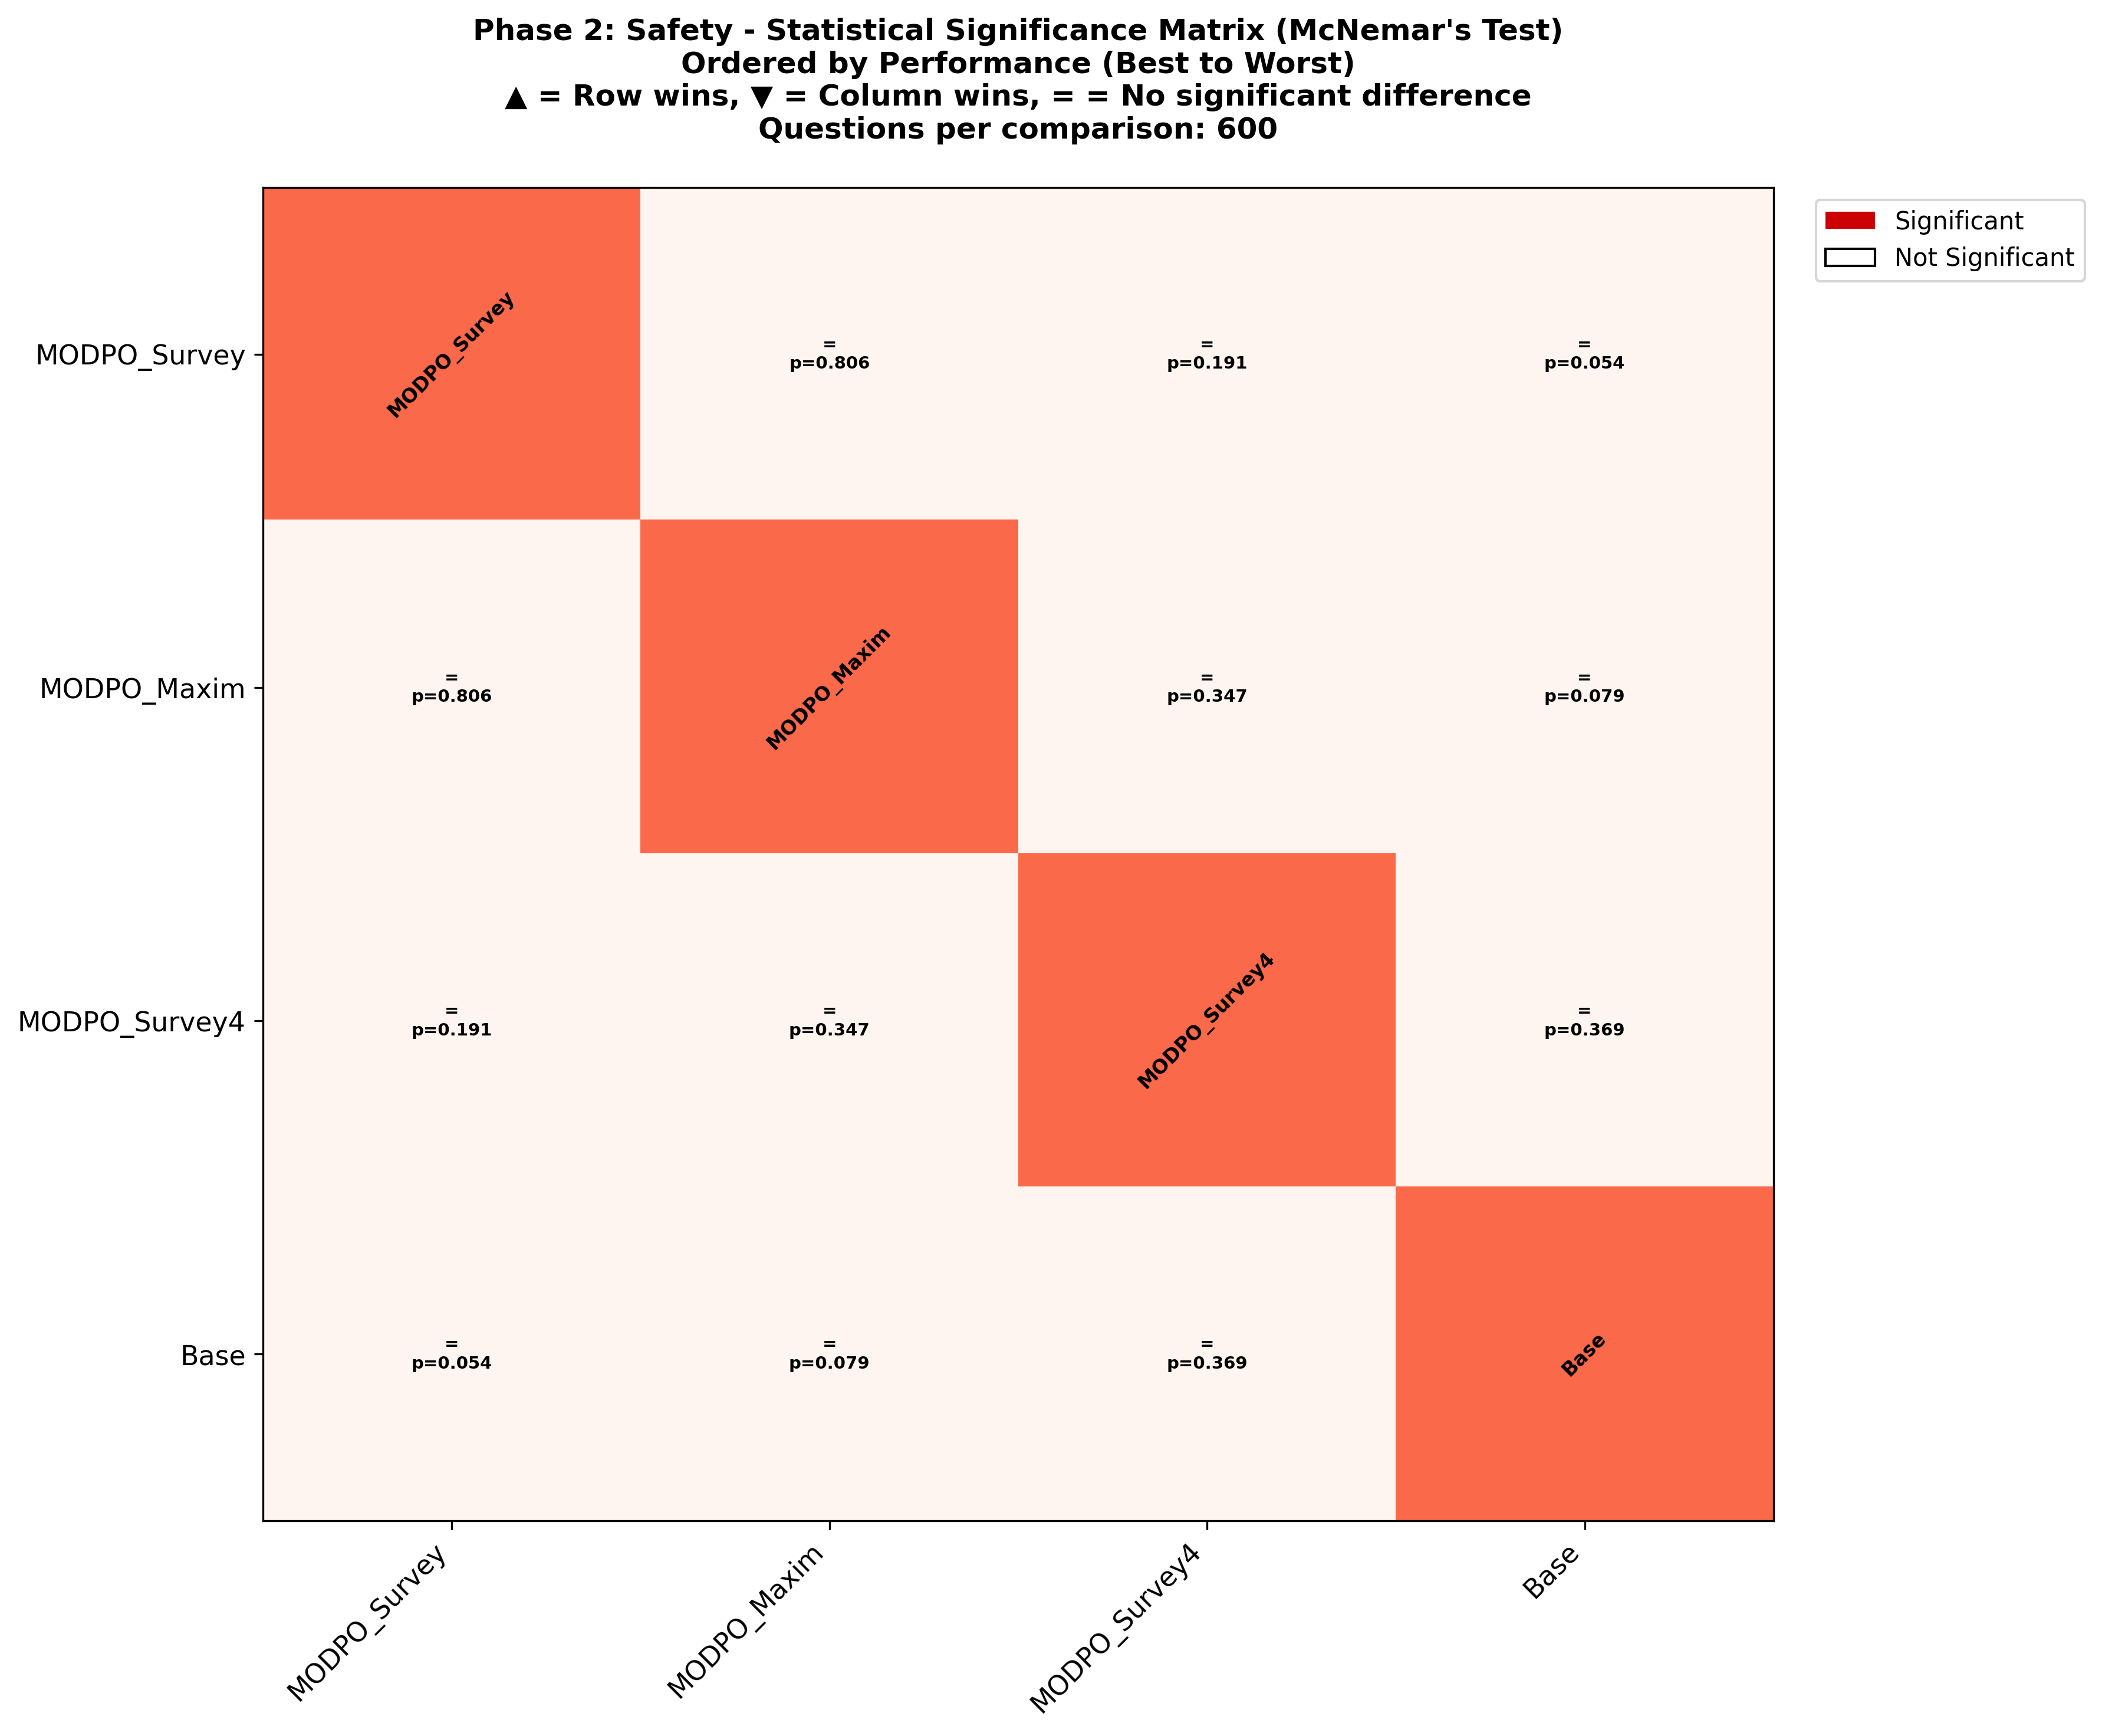}
        \caption{Safety}
    \end{subfigure}
    \caption{Statistical significance matrices using McNemar's test ($\alpha$=0.05, n=600). $\triangle$ = row wins, $\nabla$ = column wins, = = no significant difference.}
    \label{fig:phase2_significance}
\end{figure}

Overall preference evaluation showed clear statistical differentiation. MODPO\_Survey significantly outperformed all other models (all $p<0.001$), including both MODPO\_Survey4 and MODPO\_Maxim. MODPO\_Survey4 significantly beat MODPO\_Maxim ($p<0.001$) and Base ($p<0.001$). MODPO\_Maxim significantly beat Base ($p<0.001$). Every comparison reached statistical significance, establishing a clear performance hierarchy: therapeutic-specific criteria frameworks consistently and reliably outperform general communication principles.

Safety evaluation revealed no statistically significant differences in any pairwise comparison ($p>0.05$). While MODPO\_Survey achieved numerically higher safety scores than both MODPO\_Maxim (52.3\% vs 51.6\%) and MODPO\_Survey4 (52.3\% vs 49.1\%), and all three trained models achieved win rates above 50\% against Base (51.8-53.7\%), none reached significance.

\subsubsection{Criterion Quality versus Quantity}

The comparison between MODPO\_Survey4 and MODPO\_Maxim—both using exactly four criteria plus safety—isolates criterion quality while controlling for quantity. MODPO\_Survey4 significantly outperformed MODPO\_Maxim (61\% vs 38\%, $p<0.001$), yielding a 10.2 percentage point advantage on average rating. This demonstrates that therapeutic-specific criteria (Empathy, Self-Motivated Change, Trust/Rapport, Patient Autonomy) produce substantially better responses than general communication principles (Quantity, Quality, Relation, Manner) when frameworks contain the same number of criteria. The advantage derives from criterion quality—specifically, from criteria designed for therapeutic contexts rather than general conversation.

Beyond demonstrating quality over quantity, results also establish the value of our complete five-criterion framework. MODPO\_Survey significantly outperformed MODPO\_Survey4 on overall preference (57.3\% vs 42\%, $p<0.001$), demonstrating that including Active Listening as a fifth criterion meaningfully improved therapeutic response quality. On safety, MODPO\_Survey achieved 52.7\% versus MODPO\_Survey4's 47.3\% in direct comparison, indicating that adding the fifth criterion maintained safety signal strength without degradation. This finding confirms that our complete therapeutic criteria framework captures important aspects of therapeutic communication that reduced frameworks miss.

\subsection{Human Evaluation}

\begin{figure}[h]
  \centering
  \includegraphics[width=0.95\linewidth]{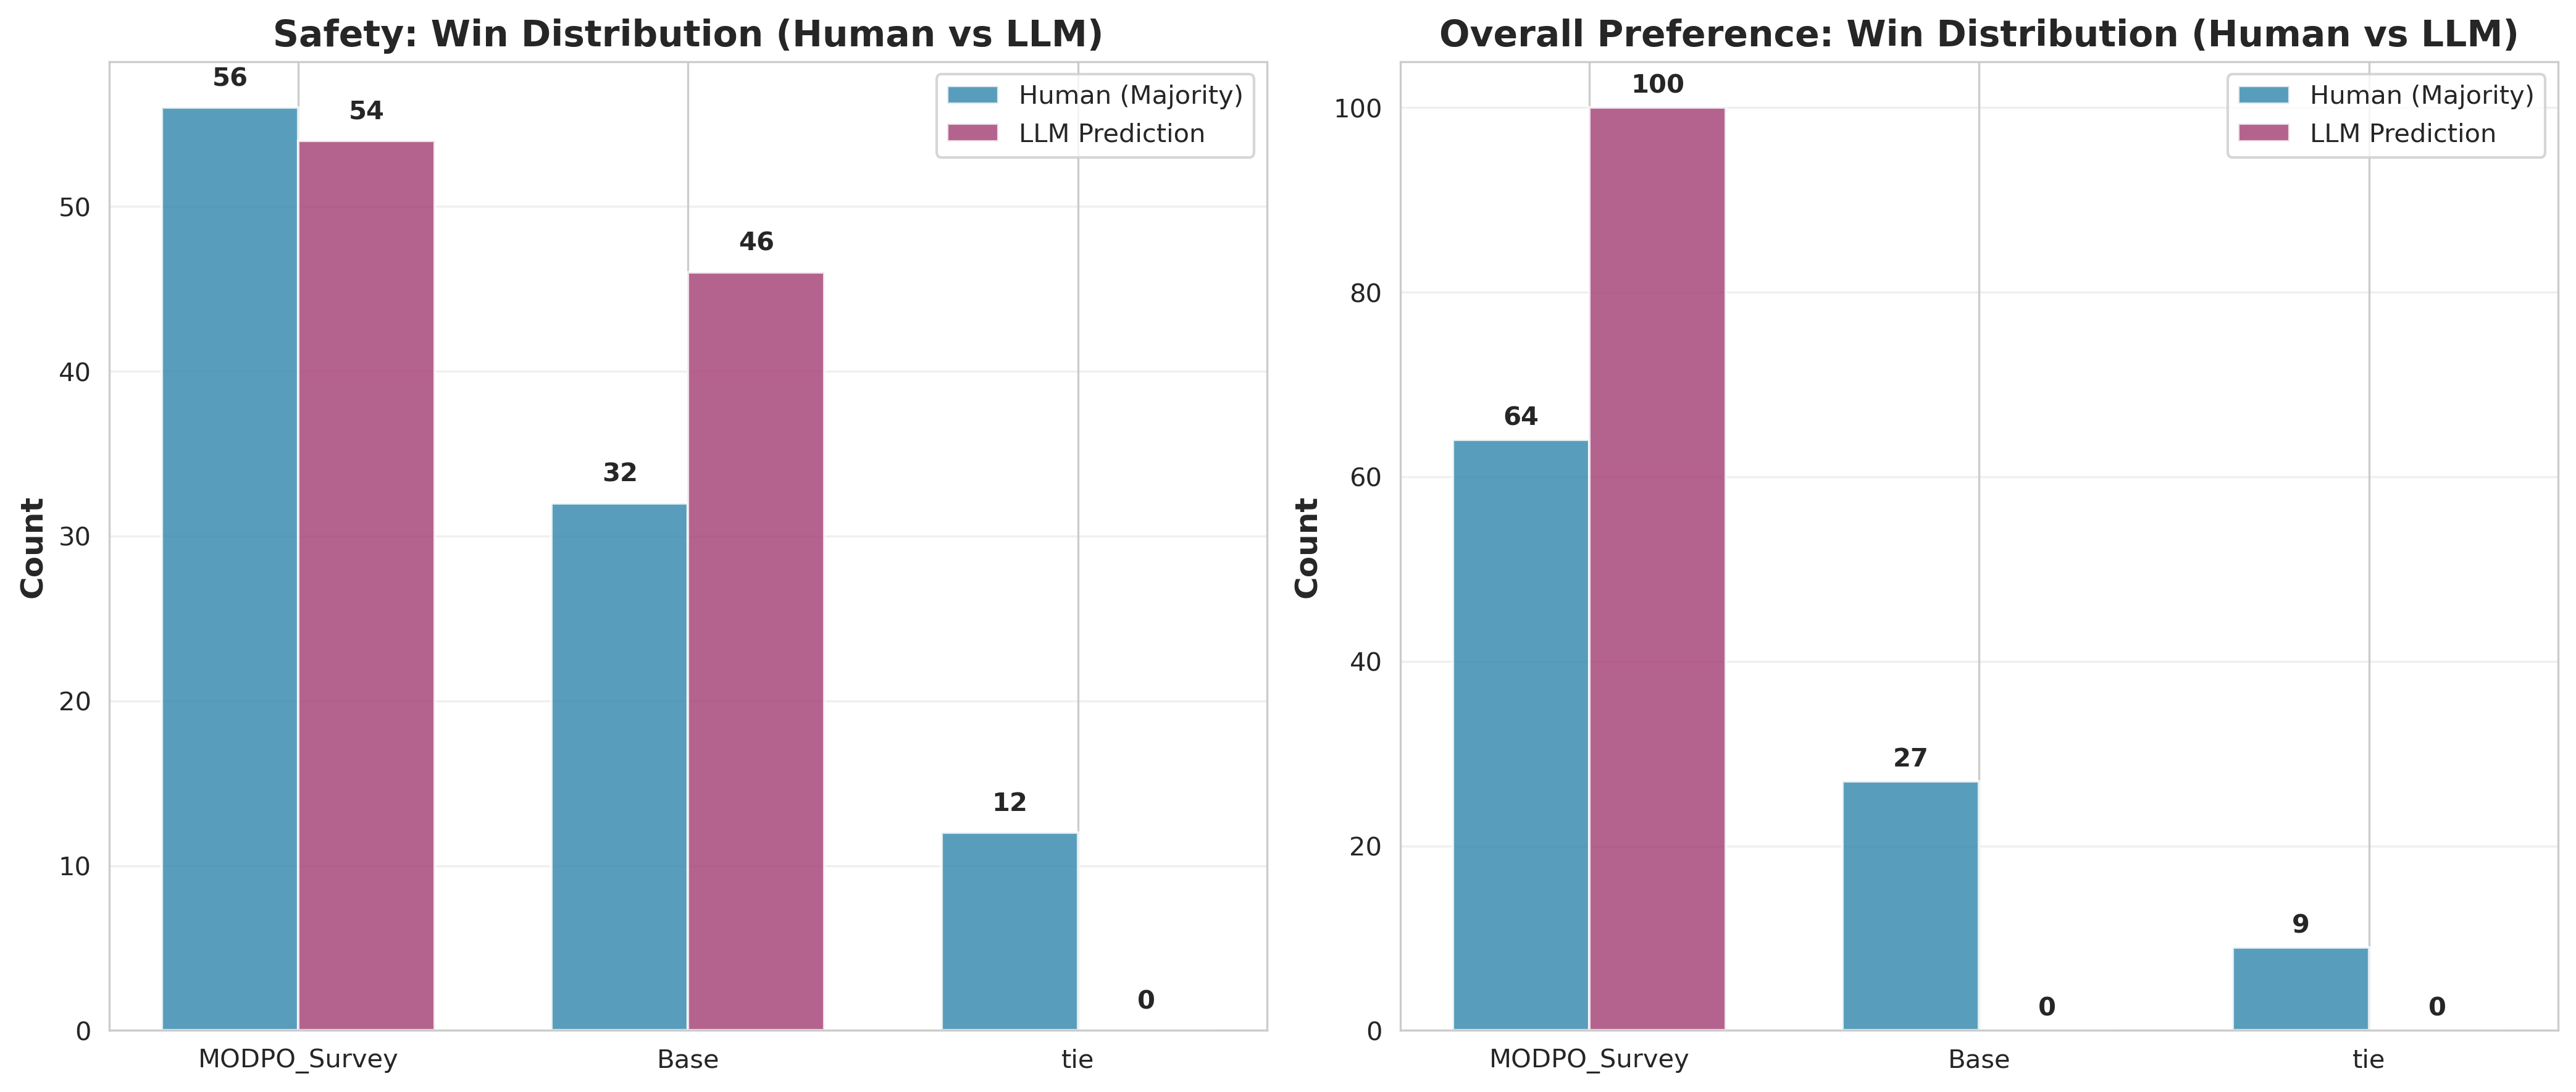}
  \caption{\textbf{Win distribution (human majority vs LLM).} Counts of MODPO\_Survey, base\_model, and tie outcomes under clinician-majority labels (blue) and LLM predictions (purple).}
  \label{fig:win_distributions}
\end{figure}

Figure~\ref{fig:win_distributions} contrasts the win distributions induced by clinician-majority judgments and by the LLM evaluator for Safety and Overall Preference. For both Safety and Overall Preference, clinicians and the LLM consistently select MODPO\_Survey as the preferred model, indicating agreement on the direction of improvement. For Safety, clinician evaluation does not reduce this preference; on the contrary, MODPO\_Survey is favored at least as often—and slightly more often—under clinician-majority judgments than under the LLM evaluator.

\subsection{Hyperparameter Configurations}

Table~\ref{tab:hyperparameters} presents the optimized hyperparameters for all trained models across both experimental phases.

\begin{table}[h]
\centering
\caption{Optimized hyperparameters for all trained models}
\label{tab:hyperparameters}
\begin{tabular}{lcccccc}
\toprule
\textbf{Model} & \textbf{LoRA Rank} & \textbf{LoRA Alpha} & \textbf{Learning Rate} & \textbf{Batch Size} & \textbf{Epochs} & \textbf{Beta} \\
\midrule
\multicolumn{7}{l}{\textit{Phase 1: Training Methodology Validation}} \\
SFT\_Empathy & 16 & 32 & 5e-5 & 8 & 3 & - \\
DPO\_Empathy & 32 & 64 & 1e-5 & 4 & 2 & 0.1 \\
MODPO\_Empathy & 32 & 64 & 1e-5 & 4 & 2 & 0.1 \\
Joint-Loss DPO & 32 & 64 & 1e-5 & 4 & 2 & 0.1 \\
DPO\_Soup & 32 & 64 & 1e-5 & 4 & 2 & 0.1 \\
\midrule
\multicolumn{7}{l}{\textit{Phase 2: Criteria Framework Comparison}} \\
MODPO\_Survey & 32 & 64 & 1e-5 & 4 & 2 & 0.1 \\
MODPO\_Survey4 & 32 & 64 & 1e-5 & 4 & 2 & 0.1 \\
MODPO\_Maxim & 32 & 64 & 1e-5 & 4 & 2 & 0.1 \\
\bottomrule
\end{tabular}
\end{table}

\textbf{Notes:} All models used LoRA dropout of 0.1, gradient accumulation steps of 4, and warmup ratio of 0.1. Beta refers to the KL-divergence penalty coefficient used in DPO and MODPO training. SFT\_Empathy used standard cross-entropy loss without a beta parameter.

\subsection{Computational Resources}

All models were trained on [SPECIFY: e.g., NVIDIA A100 40GB GPUs / V100 32GB / etc.]. 

\textbf{Training Times:}
\begin{itemize}
    \item SFT models: approximately [X] hours
    \item DPO/MODPO models: approximately [Y] hours  
    \item DPO\_Soup (two parallel models): approximately [Z] hours total
\end{itemize}

Total computational cost across all experiments: approximately [TOTAL] GPU-hours.

\subsection{Reward Model Performance}

Table~\ref{tab:reward_models} presents validation accuracies for all reward models used in multi-objective training.

\begin{table}[h]
\centering
\caption{Reward model validation accuracies}
\label{tab:reward_models}
\begin{tabular}{lc}
\toprule
\textbf{Criterion} & \textbf{Validation Accuracy} \\
\midrule
Empathy & 0.XX \\
Safety & 0.XX \\
Active Listening & 0.XX \\
Self-Motivated Change & 0.XX \\
Trust/Rapport & 0.XX \\
Patient Autonomy & 0.XX \\
Quantity (Maxim) & 0.XX \\
Quality (Maxim) & 0.XX \\
Relation (Maxim) & 0.XX \\
Manner (Maxim) & 0.XX \\
\bottomrule
\end{tabular}
\end{table}

\textbf{Notes:} All reward models used RoBERTa-large architecture fine-tuned using Optuna hyperparameter optimization across 20 trials. Models were trained on best-worst preference pairs with 10\% validation split.
